# Supplementary material for: Non-normality Can Facilitate Pulsing in Biomolecular Circuits
Source: arXiv:1710.07841 ancillary file (2018-06-02)
Supplement: Supplementary file 1 [file Sup_NonNormality_IET_SysBio_revised.pdf]

# Non-normality Can Facilitate Pulsing in Biomolecular Circuits: Supplementary Material

Abhilash Patel, Shaunak Sen[1]
Department of Electrical Engineering,
Indian Institute of Technology Delhi, India
Email: [1]shaunak.sen@ee.iitd.ac.in

## Table of Contents

S1 Mathematical Background of Non-Normality: pp2
S2 Non-normality in Three Node Random Networks:pp4
S3 Circuits information from two node screen:pp6

## S1 Mathematical Background of Non-Normality

*Definition-1: [1]* Let $A \in \mathbb{C}^{N\times N}$ and $\epsilon > 0$ be arbitrary scalar. The pseudospectrum $\sigma_\epsilon(A)$ of $A$ is the set $s \in \mathbb{C}$ such that

$$\|(sI - A)^{-1}\| \geq \epsilon^{-1},$$

where $\|(sI - A)^{-1}\|$ is called as the resolvent of $A$ at $s$.
*Definition-2: [1]* The $\epsilon$-pseudospectral abscissa is the supremum of the real parts of $z \in \sigma_\epsilon(A)$,

$$\gamma_\epsilon = \sup_{z\in\sigma_\epsilon(A)} Re(s).$$

**Theorem 1.** *[2] For an autonomous system $\dot{x} = Ax(t)$, where $x \in \mathbb{R}^n$, $A \in \mathbb{R}^{n\times n}$, and $\sigma(A) < 0$ state solution depends on transition matrix $\Phi(t, t_0) = e^{A(t-t_0)}$ and the lower bound of the maximum transient growth can be bounded as*

$$\sup_{t\geq 0} \|\Phi(t)\| \geq \frac{\gamma_\epsilon(A)}{\epsilon},$$

*and the upper bound of the transient growth can be quantify as,*

$$\sup_{t\geq 0} \|\Phi(t)\| \leq \frac{L_\epsilon(A)}{2\pi\epsilon} e^{\gamma_\epsilon t},$$

*where $L_\epsilon$ is the contour of the pseudospectrum.*

**Proof:** The proof is adopted from [1] for the lower bound and [3] for the upper bound.
*Lower Bound:* For any $z \in \sigma_\epsilon$, $Re(z) > 0$

$$\begin{aligned}
\epsilon^{-1} &\leq \|(zI - A)^{-1}\| = \|\int_0^\infty e^{tA} e^{-zt} dt\| = \int_0^\infty \|e^{tA}\|\|e^{-zt}\| dt \\
&\leq M \int_0^\infty e^{Re(z)tdt} \leq \frac{M}{Re(z)} \qquad (\|e^{tA}\| < M)
\end{aligned}$$

$$\sup_{t\geq 0} \|\Phi(t)\| \geq \frac{\sigma_\epsilon(A)}{\epsilon}$$

*Upper Bound:* From Cauchy-integral formula for matrices ($f(A) = \frac{1}{2\pi i}\int_\Gamma f(z)(z - A)^{-1} dz$, where $f$ is analytic), along the pseudospectrum

$$\begin{aligned}
\|f(A)\| =& \|\frac{1}{2\pi i}\int_{\sigma_\epsilon} f(z)(z - A)^{-1} dz\| \leq \|\frac{1}{2\pi i}\| \int_{\sigma_\epsilon} \|f(z)\|\|(z - A)^{-1}\|\|dz\| \leq \frac{1}{2\pi\epsilon}\int_{\sigma_\epsilon} \|f(z)\|\|dz\| \\
\leq& \frac{1}{2\pi\epsilon} \sup_{z\in\sigma_\epsilon} |f(z)| \int_{\sigma_\epsilon} \|dz\| \leq \frac{1}{2\pi\epsilon} \sup_{z\in\sigma_\epsilon} |f(z)| L_\epsilon
\end{aligned}$$

For $f(A) = e^{At}$,

$$\sup_{t\geq 0} \|\Phi(t)\| \leq \frac{L_\epsilon(A)}{2\pi\epsilon} e^{\gamma_\epsilon t}.$$

### Proof of condition in Eqn. (8)

The sufficient condition for transient growth is $\frac{dr}{dt}\Big|_{t=t_0} > 0$.

$$r(t) = \frac{\|\delta z(t)\|}{\|\delta z(t_0)\|} = \frac{\|e^{A(t-t_0)}\delta z(t_0)\|}{\|\delta z(t_0)\|} = \frac{\|I + A(t - t_0) + A^2\frac{(t-t_0)^2}{2!} + O(t^3)\|}{\|\delta z(t_0)\|}$$

For transient growth of the state, the condition

$$\left.\frac{dr}{dt}\right|_{t=t_0} > 0,$$

shows the potential of a pulsing output. The maximum value of the slope can be calculated, for the system with $\sigma(A) < 0$, where $\sigma(.)$ is the eigenspectrum, as

$$W(A) = \sigma_{\max}(A + A^T) > 0.$$

**Non-normality can only alter the sign of eigenvalue and numerical abssica**

For nominal system $A$, the right and left eigenvector is $v_0, u_0$ for eigenvalue $\lambda_0$. The $\|v_0\| = \|u_0\|$ is scaled to be unity. Let $E = \epsilon A^T$ and perturbed matrix becomes $A_p = A + A^T$ for $\epsilon = 1$. We can study how the eigenvectors can drift the eigenvalue to right half for $\epsilon = 1$ and to have transient growth. Let the perturbation changes the eigenvector to $v = v_0 + v_1\epsilon + v_2\epsilon^2 + ...$ and eigenvalue to $\lambda = \lambda_0 + \lambda_1\epsilon + \lambda_2\epsilon^2 + ...$

$$\begin{aligned} &A_p v = \lambda v \\ &(A + \epsilon A^T)(v_0 + \epsilon v_1 + \epsilon^2 v_1 + ...) = (\lambda_0 + \lambda_1\epsilon + \lambda_2\epsilon^2 + ...)(v_0 + \epsilon v_1 + \epsilon^2 v_1 + ...) \end{aligned} \tag{1}$$

Comparing the coefficient of $\epsilon, \epsilon^2, ...$ and spproximated with $O(\epsilon)$.

$$\begin{aligned} &Av_0 = \lambda_0 v_0 \quad \text{and} \quad A^T v_0 + Av_1 = \lambda_0 v_1 + \lambda_1 v_0 \\ &u_0 A^T v_0 + u_0 A v_1 = \lambda_0 u_0 v_1 + \lambda_1 u_0 v_0 \\ &u_0 A^T v_0 + \lambda_0 u_0 v_1 = \lambda_0 u_0 v_1 + \lambda_1 u_0 v_0 \\ &v_1 = \frac{u_0 A^T v_0}{u_0 v_0} \end{aligned} \tag{2}$$

Now, the eigenvalue becomes

$$\lambda = \lambda_0 + \frac{u_0 A^T v_0}{u_0 v_0}\epsilon$$

If we take the lower bound and put $\epsilon = 1$,

$$\lambda_0 + sv_m(A)\frac{\|u_0\|\|v_0\|}{\|u_0 v_0\|} = \lambda_0 + sv_m(A)\frac{1}{\cos\theta}$$

For normal matrices, $u_0 v_0 = 1$ and so the perturbation can not change the sign of eigenvalue.

## S2 Non-normality in Three Node Random Networks

The topologies presented below have been identified to pulse in [4]. Here, we have investigated the role of non-normality in these, finding that all of them have non-normal dynamics. In the table below, we note the topology, the pulsed response of the full mathematical model, the pseudospectrum plot and fold change, the numerical abscissa $W$, and the transfer function including system zero.

The first circuit is the one analyzed in the main text.

All other circuits except numbers 1 and 2 have complex eigenvalues indicating that the response has an oscillatory character whose envelope decays. Functionally, these are similar to a pulse. These have zeros close to the origin indicating that they exhibit a pulsed response for a step change in input. All of them should have a pulse as estimated from the pseudospectrum analysis as the corresponding $Fold_\epsilon > 1$, Some of them have $W < 0$, and still pulse. This is because the $W > 0$ condition for pulsing is a sufficient condition and hence conservative.

The circuit 2 has a zero away from the origin, yet the response shows a some aspects of pulse. This is detected by the pseudospectral analysis (as well as a consideration of the eigenvectors, please see below). In this case, all eigenvalues are real.

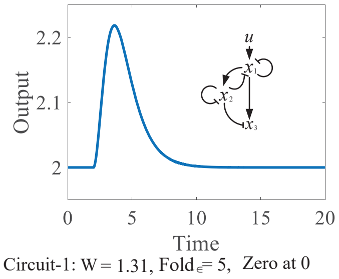

Circuit-1: W = 1.31, Fold$_\epsilon$= 5, Zero at 0

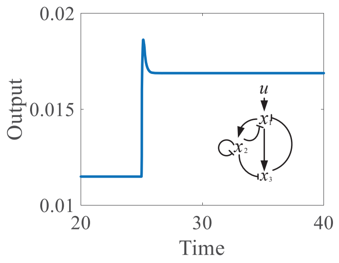

Circuit-2: W = -6.9, Fold$_\epsilon$= 1.07, Zero at -3.5

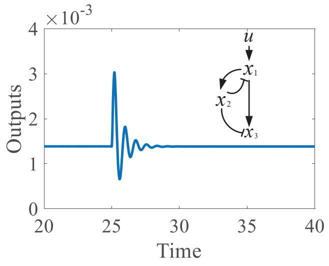

Circuit-3:W= 38.66, Fold$_\epsilon$= 1.002, Zero = 0.01

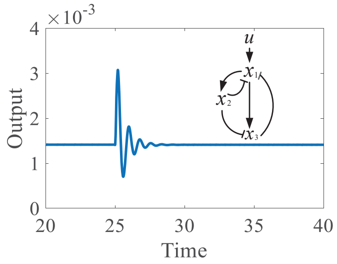

Circuit-4:W= 38.66, Fold$_\epsilon$= 1.002, Zero at 0.009

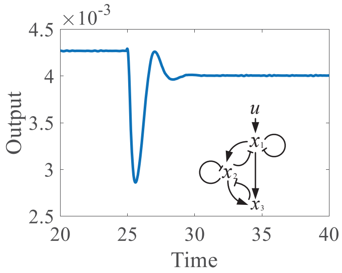

Circuit-5:W= 13.04, Fold$_\epsilon$= 1.04, Zero at 0.201

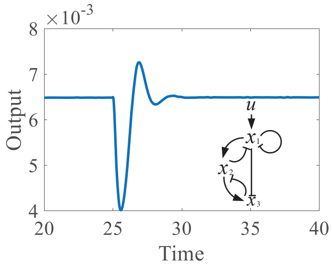

Circuit-6:W = 11.97, Fold$_\epsilon$= 1.09, Zero at 0.002

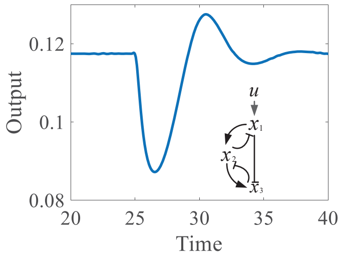

Circuit-7: W= 47.66, Fold$_\epsilon$= 5.75, Zero at -0.01

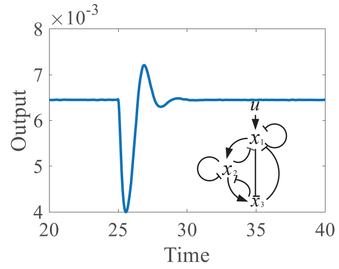

Circuit-8: W= 11.99, Fold$_\epsilon$= 2.94, Zero at -0.007

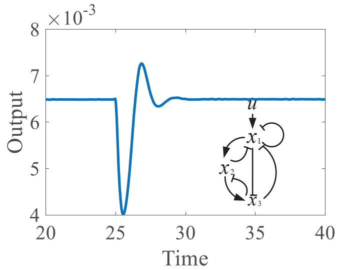

Circuit-9:W= 11.97, Fold$_\epsilon$= 2.93, Zero at 0.002

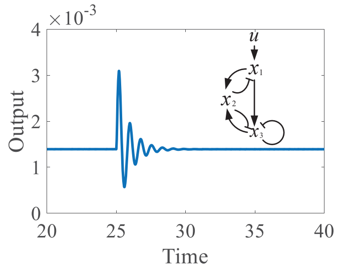


Circuit-10:W=40.19,Fold$_{\epsilon}$=1.002, Zero at 0.003

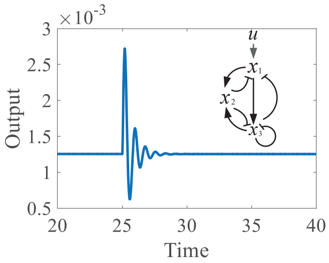


Circuit-11:W=38.65, Fold$_{\epsilon}$=1.001,Zero at 0.004

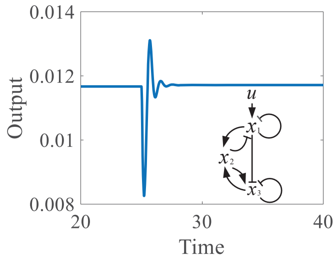


Circuit-12:W= -3.70, Fold$_{\epsilon}$= 1.03, Zero at 0.04

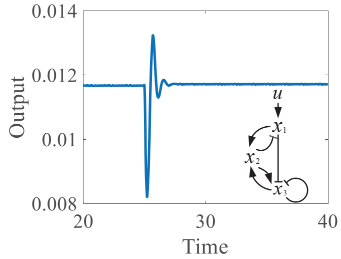


Circuit-13:W= -3.27, Fold$_{\epsilon}$= 1.03, Zero at 0.04

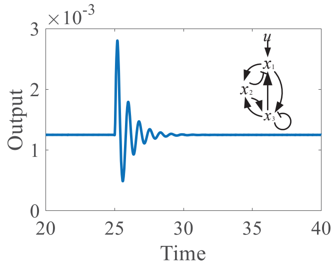


Circuit-14:W= 40.49, Fold$_{\epsilon}$=1.004,Zero at 0.004

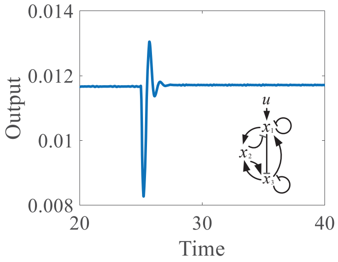


Circuit-15:W= -3.77, Fold$_{\epsilon}$ = 1.03,Zero at 0.04

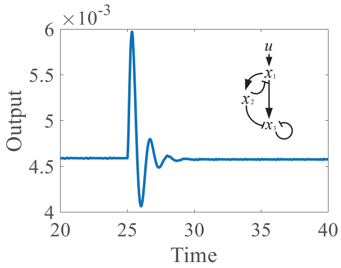


Circuit-16:W= -0.34,Fold$_{\epsilon}$= 1.002,Zero at 0.03

Table 1: Analysis of 3-node networks (topology inset)

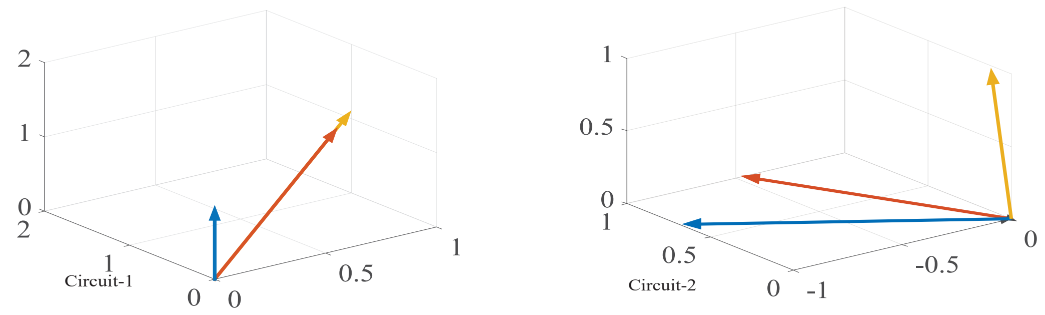


(a) (b)

Figure 1: Eigenvector for circuits 3-15 not shown as they are complex eigenvectors.

# S3 Circuits information from two node screen

The circuits presented below are from two node screen. There are total 810 possible circuits but those with issues such as non-covergence due to instability or low computational accuracy are removed from the studies. These 509 circuits are presented below. In connections box, -1 represents inhibition, 1 represents activation and 0 no regulation between. Highlighted 21 circuits belong to the set of circuits where non-normality criteria could not satisfied but non-normality is observed from angle between eigenvectors.

| | | | | | | | | | | Connections | | | | Parameters | | | |
|---|---|---|---|---|---|---|---|---|---|---|---|---|---|---|---|---|---|
| Sl Num | Step Input | Initial Cond. | W(A) | Fold | Poles | | cos (angle between eigenvectors) | Zeros | | x to x | y to x | x to y | y to y | k1 | k2 | k3 | k4 |
| 1 | Pulse | Pulse | 2.673 | 2.344 | -4.646 | -1.202 | 0.915 | -0.936 | -1.991 | -1 | -1 | -1 | -1 | 1.437 | 1.991 | 0.167 | 0.936 |
| 2 | Pulse | Pulse | 11.100 | 4.520 | -2.995 | -0.251 | 0.982 | -0.173 | -1.450 | -1 | -1 | -1 | -1 | 0.188 | 1.450 | 1.824 | 0.173 |
| 3 | Pulse | Pulse | -1.247 | 1.116 | -2.662 | -0.746 | 0.463 | -0.599 | -1.105 | -1 | -1 | -1 | -1 | 1.040 | 1.105 | 1.370 | 0.599 |
| 4 | Pulse | Pulse | -0.954 | 1.052 | -0.547 | -3.04 | 0.322 | -1.397 | -0.397 | -1 | -1 | -1 | -1 | 1.204 | 0.397 | 1.314 | 1.397 |
| 5 | Pulse | Pulse | -0.649 | 1.096 | -0.438 | -2.577 | 0.427 | -1.192 | -0.315 | -1 | -1 | -1 | -1 | 0.919 | 0.315 | 0.844 | 1.192 |
| 6 | Pulse | Pulse | -1.297 | 1.025 | -3.638 | -0.688 | 0.227 | -0.502 | -1.661 | -1 | -1 | -1 | -1 | 0.645 | 1.661 | 0.245 | 0.502 |
| 7 | Pulse | Pulse | -2.730 | 1.048 | -1.441 | -4.422 | 0.309 | -1.622 | -1.310 | -1 | -1 | -1 | -1 | 1.875 | 1.310 | 1.506 | 1.622 |
| 8 | Pulse | Pulse | 10.270 | 6.080 | -1.838 | -0.376 | 0.993 | -0.278 | -0.829 | -1 | -1 | -1 | -1 | 0.097 | 0.829 | 1.451 | 0.278 |
| 9 | Pulse | Pulse | -1.295 | 1.019 | -0.678 | -3.656 | 0.199 | -1.673 | -0.494 | -1 | -1 | -1 | -1 | 1.265 | 0.494 | 1.680 | 1.673 |
| 10 | Pulse | Pulse | 0.671 | 1.400 | -1.587 | -0.025 | 0.729 | -0.016 | -0.790 | -1 | -1 | -1 | -1 | 0.906 | 0.790 | 1.923 | 0.016 |
| 11 | Pulse | Pulse | 141.968 | 29.428 | -2.023 | -0.067 | 1.000 | 0.000 | -0.976 | -1 | -1 | -1 | 0 | 0.797 | 0.976 | 1.236 | 0.140 |
| 12 | Pulse | Pulse | 28.065 | 8.835 | -2.741 | -0.114 | 0.996 | 0.000 | -1.308 | -1 | -1 | -1 | 0 | 0.285 | 1.308 | 0.437 | 0.238 |
| 13 | Pulse | Pulse | 3.048 | 2.618 | -0.27 | -2.126 | 0.940 | -0.001 | -0.331 | -1 | -1 | -1 | 0 | 0.086 | 0.331 | 1.022 | 1.735 |
| 14 | Pulse | Pulse | 9666.534 | 303.781 | -0.218 | -1.667 | 1.000 | 0.000 | -0.270 | -1 | -1 | -1 | 0 | 1.533 | 0.270 | 0.130 | 1.345 |
| 15 | Pulse | Pulse | -0.504 | 1.017 | -2.356 | -0.272 | 0.193 | 0.000 | -0.991 | -1 | -1 | -1 | 0 | 0.964 | 0.991 | 0.627 | 0.647 |
| 16 | Pulse | Pulse | 4.049 | 2.961 | -2.005 | -0.166 | 0.955 | 0.000 | -0.901 | -1 | -1 | -1 | 0 | 1.818 | 0.901 | 1.497 | 0.371 |
| 17 | Pulse | Pulse | 2.729 | 2.717 | -0.295 | -1.856 | 0.947 | 0.000 | -0.414 | -1 | -1 | -1 | 0 | 0.170 | 0.414 | 1.118 | 1.323 |
| 18 | Pulse | Pulse | 838.558 | 87.289 | -0.073 | -0.964 | 1.000 | 0.000 | -0.080 | -1 | -1 | -1 | 0 | 1.878 | 0.080 | 0.327 | 0.876 |
| 19 | Pulse | Pulse | -0.254 | 2.026 | -0.141 | -1.018 | 0.249 | 0.000 | -0.180 | -1 | -1 | -1 | 0 | 0.651 | 0.180 | 1.621 | 0.799 |
| 20 | Pulse | Pulse | 137.500 | 11717.392 | -3.092 | -0.478 | 1.000 | 0.000 | -1.134 | -1 | -1 | -1 | 0 | 1.311 | 1.134 | 0.006 | 1.303 |
| 21 | Pulse | Pulse | -1.226 | 1.018 | -3.707 | -0.642 | 0.192 | -0.321 | No Zero | -1 | -1 | 0 | -1 | 0.173 | 1.854 | 0.297 | 0.321 |
| 22 | Pulse | Pulse | -0.672 | 1.020 | -2.699 | -0.362 | 0.207 | -0.181 | No Zero | -1 | -1 | 0 | -1 | 1.435 | 1.350 | 0.717 | 0.181 |
| 23 | Pulse | Pulse | -2.974 | 1.017 | -1.491 | -1.789 | 0.236 | -0.895 | No Zero | -1 | -1 | 0 | -1 | 0.016 | 0.746 | 1.577 | 0.895 |
| 24 | Pulse | Pulse | -3.556 | 1.039 | -3.223 | -1.809 | 0.289 | -0.905 | No Zero | -1 | -1 | 0 | -1 | 0.199 | 1.612 | 1.319 | 0.905 |
| 25 | Pulse | Pulse | -3.510 | 1.912 | -2.106 | -2.586 | 0.914 | -1.293 | No Zero | -1 | -1 | 0 | -1 | 1.067 | 1.053 | 1.259 | 1.293 |
| 26 | Pulse | Pulse | -2.778 | 1.286 | -3.204 | -1.645 | 0.658 | -0.823 | No Zero | -1 | -1 | 0 | -1 | 0.384 | 1.603 | 0.393 | 0.823 |
| 27 | Does not pulse | Pulse | 12.264 | 5.421 | -1.089 | -3.713 | 0.988 | -1.857 | No Zero | -1 | -1 | 0 | -1 | 0.471 | 0.544 | 0.017 | 1.857 |
| 28 | Pulse | Pulse | -2.333 | 1.477 | -1.857 | -1.347 | 0.811 | -0.674 | No Zero | -1 | -1 | 0 | -1 | 1.040 | 0.928 | 1.047 | 0.674 |
| 29 | Pulse | Pulse | -5.061 | 1.738 | -3.953 | -2.987 | 0.858 | -1.494 | No Zero | -1 | -1 | 0 | -1 | 0.665 | 1.977 | 0.947 | 1.494 |
| 30 | Pulse | Pulse | -1.777 | 1.218 | -3.182 | -1.136 | 0.593 | -0.568 | No Zero | -1 | -1 | 0 | -1 | 1.340 | 1.591 | 0.545 | 0.568 |
| 31 | Pulse | Pulse | -0.673 | 1.009 | -0.738 | -0.339 | 0.165 | 0.000 | No Zero | -1 | -1 | 0 | 0 | 1.435 | 0.369 | 1.667 | 0.339 |
| 32 | Pulse | Pulse | 22.012 | 11.464 | -2.889 | -1.706 | 0.999 | 0.000 | No Zero | -1 | -1 | 0 | 0 | 1.907 | 1.445 | 0.268 | 1.706 |
| 33 | Pulse | Pulse | -0.962 | 1.495 | -2.257 | -0.883 | 0.776 | 0.000 | No Zero | -1 | -1 | 0 | 0 | 1.863 | 1.128 | 0.798 | 0.883 |
| 34 | Pulse | Pulse | 160.673 | 36.407 | -1.04 | -1.896 | 1.000 | 0.000 | No Zero | -1 | -1 | 0 | 0 | 1.403 | 0.520 | 0.057 | 1.896 |
| 35 | Pulse | Pulse | -1.865 | 1.036 | -3.117 | -0.975 | 0.274 | 0.000 | No Zero | -1 | -1 | 0 | 0 | 1.992 | 1.559 | 1.979 | 0.975 |
| 36 | Pulse | Pulse | -2.542 | 1.207 | -1.857 | -1.347 | 0.636 | 0.000 | No Zero | -1 | -1 | 0 | 0 | 0.256 | 0.929 | 1.485 | 1.347 |
| 37 | Pulse | Pulse | -1.053 | 1.017 | -3.032 | -0.55 | 0.191 | 0.000 | No Zero | -1 | -1 | 0 | 0 | 1.748 | 1.517 | 1.234 | 0.550 |
| 38 | Pulse | Pulse | -0.320 | 1.000 | -3.342 | -0.161 | 0.032 | 0.000 | No Zero | -1 | -1 | 0 | 0 | 0.673 | 1.671 | 0.772 | 0.161 |
| 39 | Pulse | Pulse | -0.017 | 1.000 | -1.738 | -0.009 | 0.006 | 0.006 | No Zero | -1 | -1 | 0 | 0 | 1.731 | 0.871 | 0.344 | 0.009 |

| | | | | | | | | | | | | | | | | | |
|---|---|---|---|---|---|---|---|---|---|---|---|---|---|---|---|---|---|
| 40 | Pulse | Pulse | -0.978 | 1.889 | -1.48 | -0.883 | 0.902 | 0.000 | No Zero | -1 | -1 | 0 | 0 | 1.305 | 0.739 | 0.752 | 0.883 |
| 41 | Pulse | Pulse | -4.357 | 1.000 | -3.079 | -3.079 | 1.000 | -1.090 | -5.964 | -1 | -1 | 0 | 1 | 1.032 | 0.600 | 0.957 | 0.012 |
| 42 | Pulse | Pulse | -2.602 | 1.000 | -3.412 | -3.412 | 1.000 | -1.647 | -5.296 | -1 | -1 | 0 | 1 | 1.402 | 1.609 | 1.704 | 0.235 |
| 43 | Pulse | Pulse | -6.507 | 1.000 | -3.583 | -3.583 | 1.000 | -1.742 | -5.522 | -1 | -1 | 1 | -1 | 0.310 | 1.988 | 0.900 | 1.090 |
| 44 | Pulse | Pulse | -3.153 | 1.000 | -2.623 | -2.623 | 1.000 | -1.823 | -2.401 | -1 | -1 | 1 | -1 | 0.525 | 1.765 | 0.206 | 1.647 |
| 45 | Does not pulse | Pulse | -0.254 | 1.000 | -0.215 | -2.337 | 0.384 | -1.191 | -0.253 | -1 | -1 | 1 | -1 | 0.854 | 1.841 | 1.056 | 1.742 |
| 46 | Does not pulse | Pulse | -2.348 | 1.050 | -1.967 | -2.335 | 0.982 | -1.563 | -1.762 | -1 | -1 | 1 | -1 | 0.706 | 0.800 | 1.196 | 1.823 |
| 47 | Pulse | Pulse | -0.175 | 1.405 | -0.329 | -0.168 | 0.868 | -0.058 | -0.572 | -1 | -1 | 1 | -1 | 0.266 | 0.084 | 0.802 | 1.191 |
| 48 | Does not pulse | Pulse | -0.885 | 1.202 | -0.602 | -1.965 | 0.586 | -1.060 | -0.670 | -1 | -1 | 1 | -1 | 1.839 | 0.588 | 1.090 | 1.563 |
| 49 | Pulse | Pulse | -2.974 | 1.000 | -2.44 | -2.44 | 1.000 | -1.693 | -2.242 | -1 | -1 | 1 | -1 | 0.655 | 0.191 | 0.883 | 0.058 |
| 50 | Pulse | Pulse | -1.966 | 1.000 | -1.285 | -1.285 | 1.000 | -0.500 | -2.357 | -1 | -1 | 1 | -1 | 1.351 | 0.223 | 0.399 | 1.060 |
| 51 | Pulse | Pulse | 0.621 | 1.000 | -0.989 | -0.989 | 1.000 | 0.000 | -2.060 | -1 | -1 | 1 | -1 | 1.255 | 0.747 | 1.213 | 1.693 |
| 52 | Pulse | Pulse | -0.181 | 1.061 | -0.144 | -1.671 | 0.355 | 0.000 | -0.139 | -1 | -1 | 1 | -1 | 1.404 | 0.786 | 1.144 | 0.500 |
| 53 | Pulse | Pulse | 0.159 | 1.000 | -2.609 | -2.609 | 1.000 | 0.000 | -5.139 | -1 | -1 | 1 | 0 | 1.455 | 0.687 | 0.157 | 0.604 |
| 54 | Pulse | Pulse | -0.910 | 1.189 | -3.571 | -0.744 | 0.557 | 0.000 | -5.783 | -1 | -1 | 1 | 0 | 0.601 | 0.046 | 0.352 | 1.722 |
| 55 | Pulse | Pulse | -2.848 | 1.000 | -1.468 | -1.468 | 1.000 | 0.000 | -2.162 | -1 | -1 | 1 | 0 | 1.312 | 1.713 | 0.542 | 1.792 |
| 56 | Pulse | Pulse | 0.125 | 2.979 | -1.054 | -1.054 | 1.000 | 0.000 | -2.367 | -1 | -1 | 1 | 0 | 0.418 | 1.928 | 0.829 | 0.459 |
| 57 | Pulse | Pulse | -2.916 | 1.000 | -2.812 | -2.812 | 1.000 | 0.000 | -5.621 | -1 | -1 | 1 | 0 | 1.637 | 0.721 | 1.003 | 1.495 |
| 58 | Pulse | Pulse | -0.593 | 1.174 | -3.733 | -0.589 | 0.538 | 0.000 | -5.927 | -1 | -1 | 1 | 0 | 1.664 | 0.789 | 0.193 | 0.531 |
| 59 | Pulse | Pulse | -2.155 | 1.000 | -1.88 | -1.88 | 1.000 | 0.000 | -3.841 | -1 | -1 | 1 | 0 | 1.584 | 1.874 | 1.137 | 1.876 |
| 60 | Pulse | Pulse | -1.002 | 1.000 | -0.735 | -0.735 | 1.000 | 0.000 | -0.775 | -1 | -1 | 1 | 0 | 1.194 | 1.976 | 1.525 | 0.371 |
| 61 | Pulse | Pulse | 40.135 | 19.261 | -0.456 | -0.456 | 1.000 | 1.344 | -1.369 | -1 | -1 | 1 | 0 | 1.034 | 1.280 | 1.738 | 1.200 |
| 62 | Pulse | Pulse | 0.710 | 1.417 | -2.911 | -0.25 | 0.726 | 0.461 | -4.743 | -1 | -1 | 1 | 0 | 1.999 | 0.258 | 0.587 | 0.954 |
| 63 | Pulse | Pulse | 5.087 | 5.940 | -0.098 | -0.098 | 1.000 | 1.988 | -0.295 | -1 | -1 | 1 | 1 | 0.259 | 0.456 | 0.362 | 1.344 |
| 64 | Pulse | Pulse | 13.229 | 6.742 | -1.934 | -0.3 | 0.994 | 0.520 | -3.352 | -1 | -1 | 1 | 1 | 0.652 | 1.581 | 1.092 | 0.461 |
| 65 | Pulse | Pulse | 82.119 | 28.668 | -0.35 | -0.35 | 1.000 | 0.559 | -1.051 | -1 | -1 | 1 | 1 | 1.374 | 0.098 | 1.145 | 1.988 |
| 66 | Pulse | Pulse | 209.020 | 45.475 | -1.613 | -1.613 | 1.000 | 1.957 | -4.840 | -1 | -1 | 1 | 1 | 0.726 | 1.117 | 1.855 | 0.520 |
| 67 | Pulse | Pulse | 0.014 | 1.591 | -2.492 | -0.622 | 0.802 | 0.996 | -4.671 | -1 | -1 | 1 | 1 | 1.665 | 0.350 | 1.760 | 0.559 |
| 68 | Pulse | Pulse | 5.169 | 5.114 | -0.202 | -0.202 | 1.000 | 1.718 | -0.606 | -1 | -1 | 1 | 1 | 1.699 | 1.613 | 0.378 | 1.957 |
| 69 | Pulse | Pulse | 0.565 | 1.279 | -2.792 | -0.121 | 0.641 | 0.232 | -4.370 | -1 | -1 | 1 | 1 | 0.507 | 1.557 | 1.622 | 0.996 |
| 70 | Pulse | Pulse | 14.660 | 10.104 | -0.989 | -0.401 | 0.999 | 0.571 | -2.084 | -1 | -1 | 1 | 1 | 1.831 | 0.202 | 0.272 | 1.717 |
| 71 | Pulse | Pulse | -1.334 | 1.016 | -3.703 | -0.692 | 0.181 | No Zero | -0.346 | -1 | -1 | 1 | 1 | 0.037 | 1.457 | 1.633 | 0.232 |
| 72 | Does not pulse | Pulse | -0.068 | 1.024 | -0.038 | -0.201 | 0.313 | No Zero | -0.101 | -1 | -1 | 1 | 1 | 0.977 | 0.695 | 1.548 | 0.571 |
| 73 | Does not pulse | Pulse | -1.802 | 1.050 | -0.973 | -3.633 | 0.317 | No Zero | -1.817 | -1 | 0 | -1 | -1 | 1.649 | 0.346 | 1.727 | 1.852 |
| 74 | Pulse | Pulse | -3.703 | 1.715 | -2.424 | -3.755 | 0.843 | No Zero | -1.878 | -1 | 0 | -1 | -1 | 0.382 | 0.101 | 1.097 | 0.019 |
| 75 | Does not pulse | Does not pulse | -0.013 | 1.000 | -0.007 | -3.342 | 0.025 | No Zero | -1.672 | -1 | 0 | -1 | -1 | 1.657 | 1.817 | 1.411 | 0.487 |
| 76 | Pulse | Pulse | -2.671 | 1.390 | -3.501 | -1.728 | 0.721 | No Zero | -0.864 | -1 | 0 | -1 | -1 | 1.178 | 1.878 | 1.791 | 1.212 |
| 77 | Pulse | Pulse | -0.893 | 2.485 | -0.984 | -1.36 | 0.966 | No Zero | -0.680 | -1 | 0 | -1 | -1 | 1.585 | 1.672 | 1.120 | 0.001 |
| 78 | Does not pulse | Pulse | -1.090 | 1.034 | -0.559 | -1.153 | 0.293 | No Zero | -0.576 | -1 | 0 | -1 | -1 | 0.503 | 0.864 | 0.861 | 1.750 |
| 79 | Pulse | Pulse | -3.185 | 3.101 | -2.662 | -3.27 | 0.975 | No Zero | -1.635 | -1 | 0 | -1 | -1 | 0.135 | 0.680 | 0.354 | 0.492 |
| 80 | Pulse | Pulse | -3.252 | 1.067 | -3.878 | -1.706 | 0.364 | No Zero | -0.853 | -1 | 0 | -1 | -1 | 1.456 | 0.576 | 0.475 | 0.279 |
| 81 | Pulse | Pulse | -2.980 | 1.496 | -1.771 | -2.658 | 0.791 | No Zero | -1.329 | -1 | 0 | -1 | -1 | 0.441 | 1.635 | 0.756 | 1.331 |
| 82 | Pulse | Pulse | -0.344 | 3.515 | -0.986 | -1.182 | 0.994 | No Zero | -0.591 | -1 | 0 | -1 | -1 | 1.872 | 0.853 | 1.210 | 1.939 |
| 83 | Pulse | Pulse | -0.205 | 1.003 | -0.605 | -0.103 | 0.084 | No Zero | -0.052 | -1 | 0 | -1 | 0 | 0.729 | 1.329 | 0.630 | 1.771 |
| 84 | Does not pulse | Pulse | -2.995 | 1.220 | -1.681 | -3.135 | 0.603 | No Zero | -1.567 | -1 | 0 | -1 | 0 | 0.591 | 0.591 | 1.814 | 0.986 |
| 85 | Pulse | Pulse | -2.464 | 1.572 | -1.641 | -2.815 | 0.808 | No Zero | -1.407 | -1 | 0 | -1 | 0 | 0.414 | 0.052 | 0.340 | 0.605 |
| 86 | Does not pulse | Does not pulse | -3.984 | 1.000 | -1.992 | -3.44 | 0.024 | No Zero | -1.720 | -1 | 0 | -1 | 0 | 1.923 | 1.567 | 1.347 | 1.681 |
| 87 | Pulse | Pulse | -0.267 | 1.001 | -0.959 | -0.134 | 0.045 | No Zero | -0.067 | -1 | 0 | -1 | 0 | 0.842 | 1.407 | 0.963 | 1.641 |
| 88 | Does not pulse | Pulse | -0.537 | 1.143 | -0.341 | -1.134 | 0.533 | No Zero | -0.567 | -1 | 0 | -1 | 0 | 0.875 | 1.720 | 0.018 | 1.992 |
| 89 | Does not pulse | Pulse | -1.971 | 1.002 | -1.706 | -0.986 | 0.077 | No Zero | -0.493 | -1 | 0 | -1 | 0 | 0.550 | 0.067 | 0.304 | 0.959 |
| 90 | Does not pulse | Pulse | -1.004 | 1.378 | -1.069 | -3.832 | 0.705 | No Zero | -1.916 | -1 | 0 | -1 | 0 | 1.778 | 0.567 | 1.568 | 0.341 |
| 91 | Does not pulse | Does not pulse | -1.361 | 1.000 | -0.68 | -2.082 | 0.000 | No Zero | No Zero | -1 | 0 | -1 | 0 | 1.463 | 0.493 | 0.164 | 1.706 |

| | | | | | | | | | | | | | | | | | | |
|---|---|---|---|---|---|---|---|---|---|---|---|---|---|---|---|---|---|---|
| 92 | Does not pulse | Does not pulse | -1.361 | 1.000 | -0.68 | -2.082 | 0.000 | No Zero | -2.082 | -1 | 0 | -1 | 0 | 1.373 | 1.916 | 1.970 | 1.069 |
| 93 | Does not pulse | Does not pulse | -0.540 | 1.000 | | | 0.000 | No Zero | -1.457 | -1 | 0 | -1 | 1 | 0.257 | 1.481 | 0.782 | 0.787 |
| 94 | Does not pulse | Does not pulse | -1.761 | 1.000 | -1.18 | -0.88 | 0.000 | No Zero | -0.440 | -1 | 0 | -1 | 1 | 1.379 | 1.041 | 0.152 | 0.813 |
| 95 | Does not pulse | Does not pulse | -1.084 | 1.000 | -0.542 | -0.622 | 0.000 | No Zero | -0.311 | -1 | 0 | -1 | 1 | 0.860 | 1.319 | 0.437 | 0.162 |
| 96 | Does not pulse | Does not pulse | -3.978 | 1.000 | -3.466 | -1.989 | 0.000 | No Zero | No Zero | -1 | 0 | -1 | 1 | 0.506 | 0.440 | 0.472 | 1.620 |
| 97 | Does not pulse | Does not pulse | -3.686 | 1.000 | -2.886 | -1.843 | 0.000 | No Zero | No Zero | -1 | 0 | -1 | 1 | 1.405 | 1.757 | 1.422 | 1.322 |
| 98 | Does not pulse | Does not pulse | -1.140 | 1.000 | -3.176 | -0.57 | 0.000 | No Zero | No Zero | -1 | 0 | -1 | 1 | 0.879 | 1.126 | 1.981 | 1.915 |
| 99 | Does not pulse | Does not pulse | -0.012 | 1.000 | -0.045 | -0.006 | 0.000 | No Zero | No Zero | -1 | 0 | -1 | 1 | 0.674 | 0.311 | 0.834 | 1.109 |
| 100 | Does not pulse | Does not pulse | -2.121 | 1.000 | -2.828 | -1.06 | 0.000 | No Zero | No Zero | -1 | 0 | 0 | -1 | 0.060 | 1.733 | 1.789 | 0.994 |
| 101 | Does not pulse | Does not pulse | -0.746 | 1.000 | -3.037 | -0.373 | 0.000 | No Zero | No Zero | -1 | 0 | 0 | -1 | 0.419 | 1.443 | 1.399 | 0.921 |
| 102 | Does not pulse | Does not pulse | -4.175 | 1.000 | -2.677 | -2.087 | 0.000 | No Zero | No Zero | -1 | 0 | 0 | -1 | 0.341 | 1.589 | 1.777 | 0.285 |
| 103 | Does not pulse | Does not pulse | -1.841 | 1.000 | -2.597 | -0.921 | 0.000 | No Zero | No Zero | -1 | 0 | 0 | -1 | 1.879 | 0.001 | 0.878 | 0.022 |
| 104 | Does not pulse | Does not pulse | -4.022 | 1.000 | -2.836 | -2.011 | 0.000 | No Zero | No Zero | -1 | 0 | 0 | -1 | 0.469 | 1.414 | 1.388 | 0.530 |
| 105 | Does not pulse | Does not pulse | -2.040 | 1.000 | -2.356 | -1.02 | 0.000 | No Zero | No Zero | -1 | 0 | 0 | -1 | 0.653 | 0.186 | 0.083 | 1.519 |
| 106 | Does not pulse | Does not pulse | -1.890 | 1.000 | -2.352 | -0.945 | 0.000 | No Zero | No Zero | -1 | 0 | 0 | -1 | 0.650 | 1.044 | 1.904 | 1.338 |
| 107 | Does not pulse | Does not pulse | -3.448 | 1.000 | -1.993 | -1.724 | 0.000 | No Zero | No Zero | -1 | 0 | 0 | -1 | 0.946 | 1.299 | 1.331 | 0.460 |
| 108 | Does not pulse | Does not pulse | -0.142 | 1.000 | -3.168 | -0.071 | 0.000 | No Zero | No Zero | -1 | 0 | 0 | -1 | 1.610 | 1.006 | 0.868 | 1.418 |
| 109 | Does not pulse | Does not pulse | -0.579 | 1.000 | -2.251 | -0.29 | 0.000 | No Zero | No Zero | -1 | 0 | 0 | -1 | 1.111 | 0.510 | 0.150 | 1.178 |
| 110 | Does not pulse | Does not pulse | -2.779 | 1.000 | -1.416 | -1.389 | 0.000 | No Zero | No Zero | -1 | 0 | 0 | 0 | 1.348 | 1.176 | 1.067 | 0.945 |
| 111 | Does not pulse | Does not pulse | -2.741 | 1.000 | -2.025 | -1.37 | 0.000 | No Zero | No Zero | -1 | 0 | 0 | 0 | 0.648 | 0.862 | 1.530 | 1.993 |
| 112 | Does not pulse | Does not pulse | -2.348 | 1.000 | -3.328 | -1.174 | 0.000 | No Zero | No Zero | -1 | 0 | 0 | 0 | 0.530 | 1.584 | 0.269 | 0.071 |
| 113 | Does not pulse | Does not pulse | -3.362 | 1.000 | -3.345 | -1.681 | 0.000 | No Zero | No Zero | -1 | 0 | 0 | 0 | 0.908 | 1.126 | 0.462 | 0.290 |
| 114 | Does not pulse | Does not pulse | -0.566 | 1.000 | -1.718 | -0.283 | 0.000 | No Zero | No Zero | -1 | 0 | 0 | 0 | 1.354 | 0.708 | 1.021 | 1.389 |
| 115 | Does not pulse | Does not pulse | -0.191 | 1.000 | -3.722 | -0.096 | 0.000 | No Zero | No Zero | -1 | 0 | 0 | 0 | 1.191 | 1.012 | 1.553 | 1.370 |
| 116 | Does not pulse | Does not pulse | -1.752 | 1.000 | -2.27 | -0.876 | 0.000 | No Zero | No Zero | -1 | 0 | 0 | 0 | 0.639 | 1.664 | 1.322 | 1.174 |
| 117 | Does not pulse | Does not pulse | -1.752 | 1.000 | -2.27 | -0.876 | 0.000 | No Zero | No Zero | -1 | 0 | 0 | 0 | 0.038 | 1.674 | 0.228 | 1.681 |
| 118 | Does not pulse | Pulse | -5.361 | 2.456 | -3.185 | -3.533 | 0.967 | No Zero | -5.300 | -1 | 0 | 0 | 0 | 0.675 | 0.859 | 1.588 | 0.283 |
| 119 | Does not pulse | Pulse | -0.349 | 1.014 | -3.862 | -0.201 | 0.168 | No Zero | -0.301 | -1 | 0 | 0 | 0 | 1.216 | 1.861 | 1.273 | 0.096 |
| 120 | Does not pulse | Pulse | -2.224 | 1.181 | -3.432 | -1.322 | 0.552 | No Zero | -1.983 | -1 | 0 | 0 | 1 | 1.397 | 0.514 | 1.382 | 0.726 |
| 121 | Does not pulse | Pulse | -3.543 | 1.710 | -2.959 | -2.154 | 0.858 | No Zero | -3.230 | -1 | 0 | 0 | 1 | 1.018 | 1.135 | 0.618 | 1.494 |
| 122 | Does not pulse | Pulse | -5.537 | 2.670 | -3.793 | -3.402 | 0.972 | No Zero | -5.102 | -1 | 0 | 1 | -1 | 0.673 | 1.767 | 0.667 | 1.592 |
| 123 | Does not pulse | Pulse | -0.819 | 1.696 | -0.511 | -0.532 | 0.995 | No Zero | -0.798 | -1 | 0 | 1 | -1 | 1.610 | 0.100 | 0.805 | 1.930 |
| 124 | Does not pulse | Pulse | -0.373 | 1.021 | -3.932 | -0.227 | 0.205 | No Zero | -0.340 | -1 | 0 | 1 | -1 | 0.829 | 0.661 | 1.273 | 1.716 |
| 125 | Does not pulse | Pulse | -2.167 | 1.053 | -1.151 | -3.483 | 0.326 | No Zero | -5.224 | -1 | 0 | 1 | -1 | 1.577 | 1.077 | 1.483 | 1.479 |
| 126 | Does not pulse | Pulse | -5.079 | 4.953 | -3.802 | -3.845 | 1.000 | No Zero | -5.767 | -1 | 0 | 1 | -1 | 0.890 | 1.701 | 0.989 | 1.896 |
| 127 | Does not pulse | Pulse | -0.432 | 1.047 | -0.233 | -0.744 | 0.346 | No Zero | -1.117 | -1 | 0 | 1 | -1 | 1.596 | 0.266 | 0.476 | 0.255 |
| 128 | Does not pulse | Pulse | -2.058 | 1.377 | -1.354 | -1.118 | 0.822 | No Zero | -1.677 | -1 | 0 | 1 | -1 | 1.068 | 0.113 | 0.937 | 1.965 |
| 129 | Does not pulse | Pulse | -2.726 | 1.225 | -1.586 | -1.408 | 0.747 | No Zero | -2.112 | -1 | 0 | 1 | -1 | 1.364 | 1.742 | 0.992 | 0.575 |
| 130 | Does not pulse | Pulse | -1.247 | 1.206 | -0.843 | -2.749 | 0.583 | No Zero | -4.124 | -1 | 0 | 1 | -1 | 0.366 | 1.922 | 1.513 | 1.901 |
| 131 | Does not pulse | Pulse | -0.522 | 1.103 | -0.383 | -2.534 | 0.439 | No Zero | -3.801 | -1 | 0 | 1 | -1 | 1.343 | 0.372 | 0.580 | 0.116 |
| 132 | Does not pulse | Pulse | -2.733 | 1.125 | -1.475 | -2.993 | 0.484 | No Zero | -4.490 | -1 | 0 | 1 | 0 | 0.088 | 0.559 | 0.341 | 1.354 |
| 133 | Does not pulse | Pulse | -1.309 | 1.018 | -0.685 | -3.823 | 0.193 | No Zero | -5.734 | -1 | 0 | 1 | 0 | 1.805 | 0.704 | 0.200 | 1.586 |
| 134 | Does not pulse | Pulse | 0.395 | 1.475 | -1.131 | -0.105 | 0.777 | No Zero | -0.157 | -1 | 0 | 1 | 0 | 0.937 | 1.375 | 1.366 | 0.843 |
| 135 | Does not pulse | Pulse | -0.910 | 1.271 | -0.629 | -1.686 | 0.658 | No Zero | -2.528 | -1 | 0 | 1 | 0 | 1.319 | 1.267 | 1.050 | 0.383 |
| 136 | Does not pulse | Pulse | -0.903 | 1.015 | -1.893 | -0.464 | 0.184 | No Zero | -0.696 | -1 | 0 | 1 | 0 | 1.024 | 1.497 | 0.840 | 1.475 |
| 137 | Does not pulse | Pulse | 0.033 | 1.020 | -0.015 | -2.993 | 0.204 | No Zero | -4.489 | -1 | 0 | 1 | 0 | 1.373 | 1.911 | 0.616 | 0.685 |
| 138 | Does not pulse | Pulse | 0.033 | 1.020 | -0.015 | -2.993 | 0.204 | No Zero | -4.489 | -1 | 0 | 1 | 0 | 0.774 | 0.052 | 1.267 | 1.131 |
| 139 | Does not pulse | Does not pulse | -1.120 | 1.000 | -0.56 | -2.353 | 0.000 | No Zero | No Zero | -1 | 0 | 1 | 0 | 0.731 | 0.843 | 0.924 | 0.629 |
| 140 | Does not pulse | Does not pulse | -1.737 | 1.000 | -0.869 | -3.866 | 0.000 | No Zero | No Zero | -1 | 0 | 1 | 0 | 0.451 | 0.232 | 0.268 | 1.893 |
| 141 | Does not pulse | Does not pulse | -1.737 | 1.000 | 4.181 | -0.121 | 0.000 | No Zero | -3.866 | -1 | 0 | 1 | 0 | 0.985 | 1.496 | 0.622 | 0.015 |
| 142 | Does not pulse | Does not pulse | -2.003 | 1.000 | -1.001 | -1.749 | 0.000 | No Zero | No Zero | -1 | 0 | 1 | 1 | 1.231 | 0.715 | 1.298 | 1.692 |
| 143 | Does not pulse | Does not pulse | -2.549 | 1.000 | -1.275 | -2.696 | 0.000 | No Zero | No Zero | -1 | 0 | 1 | 1 | 0.203 | 1.177 | 1.165 | 1.044 |

| | | | | | | | | | | | | | | | | | |
|---|---|---|---|---|---|---|---|---|---|---|---|---|---|---|---|---|---|
| 144 | Does not pulse | Does not pulse | -2.549 | 1.000 | -1.275 | -2.696 | 0.000 | No Zero | No Zero | -1 | 0 | 1 | 1 | 0.909 | 1.933 | 0.365 | 1.119 |
| 145 | Pulse | Pulse | -0.068 | 1.015 | -0.043 | -1.089 | 0.186 | No Zero | -0.034 | -1 | 0 | 1 | 1 | 1.253 | 0.060 | 1.285 | 1.676 |
| 146 | Pulse | Pulse | -0.068 | 1.015 | -0.043 | -1.089 | 0.186 | -1.646 | -0.017 | -1 | 0 | 1 | 1 | 0.790 | 0.875 | 0.170 | 1.163 |
| 147 | Pulse | Pulse | -2.528 | 1.100 | -1.579 | -1.579 | 1.000 | -2.357 | -0.793 | -1 | 0 | 1 | 1 | 1.743 | 0.414 | 0.189 | 0.376 |
| 148 | Pulse | Pulse | -4.016 | 1.001 | -3.024 | -3.024 | 1.000 | -4.078 | -1.665 | -1 | 0 | 1 | 1 | 0.250 | 1.348 | 1.361 | 1.860 |
| 149 | Pulse | Pulse | 0.049 | 1.796 | -0.091 | -0.091 | 1.000 | -0.184 | -0.030 | -1 | 1 | -1 | -1 | 0.435 | 0.017 | 0.601 | 0.549 |
| 150 | Pulse | Pulse | -0.349 | 1.079 | -0.243 | -1.77 | 0.397 | -2.736 | -0.094 | -1 | 1 | -1 | -1 | 1.173 | 0.793 | 0.373 | 0.786 |
| 151 | Pulse | Pulse | -0.599 | 1.000 | -1.154 | -1.154 | 1.000 | -1.311 | -0.717 | -1 | 1 | -1 | -1 | 0.309 | 1.665 | 0.300 | 1.359 |
| 152 | Pulse | Pulse | -4.389 | 1.000 | -2.576 | -2.576 | 1.000 | -4.433 | -1.098 | -1 | 1 | -1 | -1 | 1.500 | 0.030 | 0.284 | 0.061 |
| 153 | Does not pulse | Pulse | -0.111 | 1.007 | -3.872 | -0.07 | 0.121 | -0.083 | -1.943 | -1 | 1 | -1 | -1 | 1.617 | 0.094 | 1.332 | 0.912 |
| 154 | Does not pulse | Pulse | -0.387 | 1.616 | -1.773 | -0.627 | 0.822 | -0.687 | -0.971 | -1 | 1 | -1 | -1 | 1.606 | 0.717 | 0.051 | 0.437 |
| 155 | Does not pulse | Pulse | -0.984 | 1.339 | -2.223 | -0.777 | 0.697 | -0.852 | -1.216 | -1 | 1 | -1 | -1 | 1.422 | 1.098 | 1.739 | 1.478 |
| 156 | Pulse | Pulse | -2.682 | 1.000 | -2.551 | -2.551 | 1.000 | -2.760 | -1.861 | -1 | 1 | -1 | -1 | 0.206 | 1.943 | 1.477 | 0.028 |
| 157 | Pulse | Pulse | -1.290 | 1.000 | -1.077 | -1.077 | 1.000 | -2.654 | -0.414 | -1 | 1 | -1 | -1 | 1.358 | 0.971 | 0.069 | 0.229 |
| 158 | Pulse | Pulse | -3.106 | 1.000 | -1.938 | -1.938 | 1.000 | -3.863 | -0.972 | -1 | 1 | -1 | -1 | 0.153 | 1.216 | 0.467 | 0.284 |
| 159 | Pulse | Pulse | -1.843 | 1.000 | -1.253 | -1.253 | 1.000 | -3.037 | -0.493 | -1 | 1 | -1 | 0 | 1.060 | 1.861 | 1.234 | 1.380 |
| 160 | Pulse | Pulse | -2.448 | 1.000 | -2.282 | -2.282 | 1.000 | -2.549 | -1.645 | -1 | 1 | -1 | 0 | 0.469 | 0.414 | 0.075 | 1.327 |
| 161 | Pulse | Pulse | -0.005 | 1.000 | -1.304 | -1.304 | 1.000 | -3.740 | -0.369 | -1 | 1 | -1 | 0 | 1.015 | 0.972 | 1.723 | 1.931 |
| 162 | Pulse | Pulse | -1.971 | 1.000 | -2.084 | -2.084 | 1.000 | -1.977 | -1.590 | -1 | 1 | -1 | 0 | 1.519 | 0.493 | 1.353 | 1.519 |
| 163 | Pulse | Pulse | -2.176 | 1.000 | -2.417 | -2.417 | 1.000 | -2.533 | -1.784 | -1 | 1 | -1 | 0 | 1.172 | 1.645 | 1.854 | 1.275 |
| 164 | Pulse | Pulse | -2.285 | 1.000 | -1.288 | -1.288 | 1.000 | -2.817 | -0.583 | -1 | 1 | -1 | 0 | 0.038 | 0.369 | 0.053 | 1.870 |
| 165 | Does not pulse | Pulse | -0.999 | 1.301 | -2.949 | -0.85 | 0.662 | -1.015 | -1.645 | -1 | 1 | -1 | 0 | 0.969 | 1.590 | 0.914 | 0.988 |
| 166 | Does not pulse | Pulse | 0.874 | 1.963 | -2.052 | -0.468 | 0.884 | -0.762 | -1.259 | -1 | 1 | -1 | 0 | 0.851 | 1.784 | 1.749 | 1.266 |
| 167 | Does not pulse | Pulse | 0.093 | 1.706 | -1.559 | -0.443 | 0.846 | -0.690 | -1.001 | -1 | 1 | -1 | 0 | 0.585 | 0.583 | 0.491 | 1.409 |
| 168 | Does not pulse | Pulse | 2.192 | 3.499 | -1.962 | -0.852 | 0.975 | -1.188 | -1.407 | -1 | 1 | -1 | 0 | 1.549 | 1.645 | 1.612 | 0.508 |
| 169 | Does not pulse | Pulse | 0.044 | 1.556 | -2.396 | -0.559 | 0.791 | -0.907 | -1.477 | -1 | 1 | -1 | 1 | 1.601 | 1.259 | 0.463 | 0.762 |
| 170 | Does not pulse | Pulse | 0.005 | 1.698 | -2.898 | -0.817 | 0.829 | -1.275 | -1.857 | -1 | 1 | -1 | 1 | 0.906 | 1.001 | 1.081 | 0.690 |
| 171 | Pulse | Pulse | 15.697 | 11.185 | -1.108 | -1.108 | 1.000 | -1.604 | -1.108 | -1 | 1 | -1 | 1 | 0.583 | 1.407 | 1.868 | 1.188 |
| 172 | Pulse | Pulse | 69.460 | 25.662 | -0.401 | -0.401 | 1.000 | -1.526 | -0.401 | -1 | 1 | -1 | 1 | 1.186 | 1.477 | 0.745 | 0.907 |
| 173 | Does not pulse | Pulse | 0.005 | 2.500 | -1.308 | -1.308 | 1.000 | -1.469 | -1.308 | -1 | 1 | -1 | 1 | 1.019 | 1.857 | 0.902 | 1.275 |
| 174 | Does not pulse | Pulse | 7.995 | 9.739 | -1.331 | -1.331 | 1.000 | -1.427 | -1.332 | -1 | 1 | -1 | 1 | 0.919 | 1.108 | 0.082 | 1.604 |
| 175 | Does not pulse | Pulse | 0.160 | 4.320 | -1.282 | -1.282 | 1.000 | -1.357 | -1.282 | -1 | 1 | -1 | 1 | 1.343 | 0.401 | 0.029 | 1.526 |
| 176 | Does not pulse | Pulse | -1.770 | 1.007 | -0.896 | -3.714 | 0.124 | -5.571 | No Zero | -1 | 1 | -1 | 1 | 1.135 | 1.308 | 1.269 | 1.469 |
| 177 | Does not pulse | Pulse | -0.551 | 1.039 | -2.694 | -0.326 | 0.282 | -0.489 | No Zero | -1 | 1 | -1 | 1 | 1.775 | 1.332 | 0.241 | 1.427 |
| 178 | Does not pulse | Pulse | -1.633 | 1.432 | -1.137 | -0.916 | 0.852 | -1.375 | No Zero | -1 | 1 | -1 | 1 | 0.894 | 1.282 | 1.298 | 1.357 |
| 179 | Does not pulse | Pulse | -4.676 | 2.575 | -2.706 | -2.815 | 0.992 | -4.222 | No Zero | -1 | 1 | 0 | -1 | 0.118 | 0.448 | 0.336 | 1.857 |
| 180 | Does not pulse | Pulse | -1.546 | 3.927 | -2.91 | -2.335 | 0.988 | -3.502 | No Zero | -1 | 1 | 0 | -1 | 1.030 | 1.347 | 1.336 | 0.163 |
| 181 | Does not pulse | Pulse | -0.669 | 1.018 | -0.367 | -3.722 | 0.193 | -5.583 | No Zero | -1 | 1 | 0 | -1 | 0.450 | 0.568 | 1.828 | 0.458 |
| 182 | Does not pulse | Pulse | -3.749 | 1.402 | -2.102 | -2.994 | 0.749 | -4.491 | No Zero | -1 | 1 | 0 | -1 | 0.497 | 1.353 | 1.297 | 1.407 |
| 183 | Does not pulse | Pulse | -1.450 | 1.020 | -0.749 | -2.852 | 0.208 | -4.278 | No Zero | -1 | 1 | 0 | -1 | 1.674 | 1.455 | 0.039 | 1.167 |
| 184 | Does not pulse | Pulse | -3.323 | 2.015 | -2.733 | -2.124 | 0.918 | -3.185 | No Zero | -1 | 1 | 0 | -1 | 1.842 | 0.183 | 1.109 | 1.862 |
| 185 | Does not pulse | Pulse | -3.785 | 1.103 | -1.972 | -3.313 | 0.449 | -4.969 | No Zero | -1 | 1 | 0 | -1 | 0.399 | 1.051 | 0.253 | 1.497 |
| 186 | Does not pulse | Pulse | -1.355 | 1.041 | -2.111 | -0.71 | 0.296 | -1.420 | No Zero | -1 | 1 | 0 | -1 | 0.629 | 0.374 | 1.961 | 1.426 |
| 187 | Does not pulse | Pulse | -1.418 | 1.627 | -2.87 | -1.288 | 0.816 | -2.575 | No Zero | -1 | 1 | 0 | -1 | 1.651 | 1.366 | 1.379 | 1.062 |
| 188 | Does not pulse | Does not pulse | -0.028 | 1.000 | -2.055 | -0.014 | 0.001 | -0.033 | No Zero | -1 | 1 | 0 | -1 | 0.378 | 0.986 | 1.119 | 1.657 |
| 189 | Does not pulse | Pulse | -2.437 | 1.359 | -3.333 | -1.576 | 0.704 | -3.153 | No Zero | -1 | 1 | 0 | 0 | 0.406 | 1.055 | 1.616 | 0.710 |
| 190 | Does not pulse | Pulse | -0.961 | 1.283 | -0.609 | -1.29 | 0.688 | -2.580 | No Zero | -1 | 1 | 0 | 0 | 1.096 | 1.435 | 0.405 | 1.288 |
| 191 | Does not pulse | Pulse | -0.175 | 1.096 | -0.373 | -0.111 | 0.523 | -0.221 | No Zero | -1 | 1 | 0 | 0 | 0.000 | 1.026 | 1.140 | 0.014 |
| 192 | Does not pulse | Pulse | 1.590 | 6.430 | -1.854 | -1.684 | 0.999 | -3.368 | No Zero | -1 | 1 | 0 | 0 | 1.785 | 1.666 | 1.550 | 1.576 |
| 193 | Does not pulse | Pulse | -0.748 | 1.420 | -0.46 | -0.629 | 0.869 | -1.258 | No Zero | -1 | 1 | 0 | 0 | 0.747 | 0.305 | 0.705 | 1.290 |
| 194 | Does not pulse | Pulse | -3.221 | 1.753 | -2.709 | -1.987 | 0.872 | -3.973 | No Zero | -1 | 1 | 0 | 0 | 1.864 | 0.187 | 1.478 | 0.111 |
| 195 | Does not pulse | Pulse | -1.262 | 1.698 | -1.1 | -0.822 | 0.907 | -1.644 | No Zero | -1 | 1 | 0 | 0 | 1.514 | 0.927 | 0.090 | 1.684 |

| | | | | | | | | | | | | | | | | | |
|---|---|---|---|---|---|---|---|---|---|---|---|---|---|---|---|---|---|
| 196 | Does not pulse | Does not pulse | -2.619 | 1.002 | -4.529 | -1.313 | 0.069 | -3.218 | -5.547 | -1 | 1 | 0 | 0 | 0.329 | 0.230 | 0.543 | 0.629 |
| 197 | Does not pulse | Does not pulse | -0.556 | 1.000 | -1.102 | -0.278 | 0.025 | -0.646 | -1.424 | -1 | 1 | 0 | 0 | 1.212 | 1.355 | 1.975 | 1.987 |
| 198 | Does not pulse | Pulse | -0.460 | 1.027 | -0.275 | -3.353 | 0.236 | -4.875 | -0.567 | -1 | 1 | 0 | 0 | 1.515 | 0.550 | 1.908 | 0.822 |
| 199 | Does not pulse | Does not pulse | -1.739 | 1.001 | -3.903 | -0.87 | 0.037 | -1.960 | -5.201 | -1 | 1 | 1 | -1 | 0.575 | 1.849 | 0.597 | 1.073 |
| 200 | Does not pulse | Does not pulse | -2.442 | 1.022 | -1.256 | -4.255 | 0.213 | -5.157 | -3.109 | -1 | 1 | 1 | -1 | 0.667 | 0.475 | 1.090 | 0.215 |
| 201 | Does not pulse | Does not pulse | -3.006 | 1.027 | -4.704 | -1.548 | 0.235 | -4.317 | -5.061 | -1 | 1 | 1 | -1 | 0.274 | 0.189 | 0.622 | 1.625 |
| 202 | Does not pulse | Does not pulse | -0.052 | 1.002 | -0.028 | -2.041 | 0.067 | -3.047 | -0.058 | -1 | 1 | 1 | -1 | 1.027 | 1.733 | 1.961 | 0.653 |
| 203 | Does not pulse | Pulse | -1.510 | 1.335 | -1.221 | -3.764 | 0.681 | -4.178 | -3.300 | -1 | 1 | 1 | -1 | 0.439 | 1.036 | 0.706 | 1.719 |
| 204 | Does not pulse | Pulse | -0.145 | 1.001 | -0.073 | -1.712 | 0.039 | -2.529 | -0.148 | -1 | 1 | 1 | -1 | 0.520 | 1.687 | 1.166 | 1.439 |
| 205 | Does not pulse | Pulse | -0.441 | 1.007 | -0.233 | -3.687 | 0.117 | -5.405 | -0.476 | -1 | 1 | 1 | -1 | 0.687 | 0.019 | 0.385 | 1.015 |
| 206 | Does not pulse | Pulse | -0.612 | 1.067 | -2.295 | -0.378 | 0.366 | -2.213 | -2.349 | -1 | 1 | 1 | -1 | 0.048 | 1.100 | 0.552 | 1.392 |
| 207 | Does not pulse | Pulse | -1.210 | 1.002 | -4.179 | -0.61 | 0.070 | -3.192 | -4.788 | -1 | 1 | 1 | -1 | 1.763 | 0.049 | 0.682 | 0.843 |
| 208 | Does not pulse | Pulse | 0.196 | 1.074 | -3.68 | -0.044 | 0.374 | -0.088 | -5.491 | -1 | 1 | 1 | -1 | 0.160 | 0.159 | 0.145 | 1.801 |
| 209 | Does not pulse | Pulse | -0.782 | 1.000 | -2.768 | -0.391 | 0.007 | -2.008 | -3.233 | -1 | 1 | 1 | 0 | 1.939 | 0.783 | 0.627 | 1.107 |
| 210 | Does not pulse | Pulse | 1.359 | 1.841 | -0.358 | -2.541 | 0.859 | -3.959 | -1.380 | -1 | 1 | 1 | 0 | 1.584 | 1.597 | 1.727 | 1.596 |
| 211 | Does not pulse | Pulse | 0.528 | 1.726 | -0.1 | -0.829 | 0.866 | -1.376 | -0.360 | -1 | 1 | 1 | 0 | 0.013 | 1.840 | 0.036 | 0.059 |
| 212 | Does not pulse | Pulse | -1.143 | 1.001 | -3.59 | -0.573 | 0.039 | -3.218 | -3.831 | -1 | 1 | 1 | 0 | 1.423 | 1.077 | 1.049 | 1.004 |
| 213 | Does not pulse | Pulse | -0.772 | 1.026 | -2.536 | -0.416 | 0.234 | -2.432 | -2.605 | -1 | 1 | 1 | 0 | 0.131 | 0.460 | 0.234 | 1.980 |
| 214 | Does not pulse | Pulse | 0.822 | 1.322 | -4.039 | -0.238 | 0.667 | -1.023 | -5.650 | -1 | 1 | 1 | 0 | 0.141 | 0.120 | 1.323 | 0.688 |
| 215 | Does not pulse | Pulse | 0.539 | 1.423 | -5.072 | -0.706 | 0.723 | -3.596 | -5.969 | -1 | 1 | 1 | 0 | 0.257 | 1.274 | 1.493 | 1.611 |
| 216 | Pulse | Pulse | -0.894 | 1.027 | -0.503 | -4.484 | 0.232 | -1.903 | -0.001 | -1 | 1 | 1 | 0 | 0.538 | 0.868 | 0.804 | 1.216 |
| 217 | Pulse | Pulse | -1.229 | 1.007 | -0.627 | -3.906 | 0.120 | -1.379 | 0.000 | -1 | 1 | 1 | 0 | 1.540 | 1.882 | 0.263 | 0.511 |
| 218 | Pulse | Pulse | 3.052 | 3.622 | -0.157 | -0.979 | 0.981 | -0.345 | 0.000 | -1 | 1 | 1 | 0 | 0.757 | 1.987 | 0.682 | 1.799 |
| 219 | Pulse | Pulse | 455.190 | 57.983 | -0.033 | -2.124 | 1.000 | -1.045 | 0.002 | 0 | -1 | -1 | -1 | 0.624 | 1.184 | 0.755 | 1.903 |
| 220 | Pulse | Pulse | 21.368 | 6.645 | -0.383 | -3.539 | 0.992 | -1.514 | 0.000 | 0 | -1 | -1 | -1 | 1.485 | 1.774 | 1.198 | 1.379 |
| 221 | Pulse | Pulse | 3.071 | 2.043 | -0.467 | -4.005 | 0.883 | -1.680 | -0.001 | 0 | -1 | -1 | -1 | 0.782 | 0.447 | 0.263 | 0.345 |
| 222 | Pulse | Pulse | 49.647 | 17.932 | -1.273 | -0.209 | 1.000 | -0.305 | 0.000 | 0 | -1 | -1 | -1 | 1.877 | 0.069 | 1.759 | 1.045 |
| 223 | Pulse | Pulse | -1.156 | 1.001 | -0.579 | -3.455 | 0.033 | -1.141 | 0.000 | 0 | -1 | -1 | -1 | 1.616 | 0.895 | 0.693 | 1.514 |
| 224 | Pulse | Pulse | 2.413 | 2.229 | -2.895 | -0.477 | 0.908 | -0.701 | 0.000 | 0 | -1 | -1 | -1 | 0.720 | 1.113 | 1.777 | 1.680 |
| 225 | Pulse | Pulse | 0.156 | 1.452 | -0.712 | -0.113 | 0.792 | -0.157 | 0.000 | 0 | -1 | -1 | -1 | 0.488 | 0.871 | 1.657 | 0.305 |
| 226 | Does not pulse | Pulse | -2.705 | 1.499 | -1.897 | -3.826 | 0.769 | -1.913 | No Zero | 0 | -1 | -1 | -1 | 1.516 | 1.753 | 1.004 | 1.141 |
| 227 | Pulse | Pulse | -1.679 | 1.095 | -1.054 | -0.859 | 0.549 | -0.429 | No Zero | 0 | -1 | -1 | -1 | 1.703 | 1.969 | 1.580 | 0.701 |
| 228 | Does not pulse | Pulse | 0.839 | 1.402 | -0.277 | -3.5 | 0.716 | -1.751 | No Zero | 0 | -1 | -1 | -1 | 1.004 | 0.510 | 1.020 | 0.157 |
| 229 | Pulse | Pulse | -0.599 | 1.026 | -0.994 | -0.311 | 0.255 | -0.156 | No Zero | 0 | -1 | 0 | -1 | 1.253 | 1.897 | 1.033 | 1.913 |
| 230 | Does not pulse | Pulse | -0.099 | 1.018 | -0.052 | -0.06 | 0.730 | -0.030 | No Zero | 0 | -1 | 0 | -1 | 0.544 | 1.054 | 1.822 | 0.429 |
| 231 | Does not pulse | Pulse | -0.195 | 1.115 | -0.239 | -2.489 | 0.460 | -1.244 | No Zero | 0 | -1 | 0 | -1 | 1.654 | 0.277 | 0.876 | 1.751 |
| 232 | Does not pulse | Pulse | -0.934 | 1.112 | -0.62 | -3.13 | 0.453 | -1.565 | No Zero | 0 | -1 | 0 | -1 | 1.409 | 0.994 | 1.219 | 0.156 |
| 233 | Does not pulse | Pulse | -0.886 | 1.008 | -0.562 | -0.444 | 0.205 | -0.222 | No Zero | 0 | -1 | 0 | -1 | 0.483 | 0.052 | 1.693 | 0.030 |
| 234 | Does not pulse | Pulse | -0.055 | 1.133 | -0.205 | -2.649 | 0.487 | -1.324 | No Zero | 0 | -1 | 0 | -1 | 1.101 | 0.239 | 1.176 | 1.244 |
| 235 | Pulse | Pulse | -0.154 | 1.004 | -1.864 | -0.082 | 0.100 | -0.041 | No Zero | 0 | -1 | 0 | -1 | 1.494 | 0.620 | 1.833 | 1.565 |
| 236 | Pulse | Pulse | 0.234 | 1.575 | -0.946 | -0.178 | 0.825 | 0.000 | No Zero | 0 | -1 | 0 | -1 | 0.202 | 0.562 | 1.815 | 0.222 |
| 237 | Pulse | Pulse | -0.671 | 1.002 | -0.336 | -0.572 | 0.084 | 0.000 | No Zero | 0 | -1 | 0 | -1 | 1.580 | 0.205 | 1.536 | 1.324 |
| 238 | Pulse | Pulse | 7.417 | 9.157 | -1.704 | -1.454 | 1.000 | 0.000 | No Zero | 0 | -1 | 0 | -1 | 1.546 | 1.864 | 0.354 | 0.041 |
| 239 | Pulse | Pulse | -1.074 | 1.416 | -0.621 | -0.784 | 0.871 | 0.000 | No Zero | 0 | -1 | 0 | 0 | 1.667 | 0.946 | 0.217 | 0.178 |
| 240 | Pulse | Pulse | -2.004 | 1.024 | -1.957 | -1.016 | 0.236 | 0.000 | No Zero | 0 | -1 | 0 | 0 | 0.230 | 0.336 | 1.945 | 0.572 |
| 241 | Pulse | Pulse | -0.776 | 1.038 | -0.395 | -0.536 | 0.406 | 0.000 | No Zero | 0 | -1 | 0 | 0 | 1.198 | 1.704 | 0.490 | 1.454 |
| 242 | Pulse | Pulse | -1.072 | 1.008 | -1.103 | -0.539 | 0.148 | 0.000 | No Zero | 0 | -1 | 0 | 0 | 0.802 | 0.621 | 1.308 | 0.784 |
| 243 | Pulse | Pulse | -1.096 | 1.384 | -0.62 | -0.756 | 0.874 | 0.000 | No Zero | 0 | -1 | 0 | 0 | 0.239 | 1.957 | 1.037 | 1.016 |
| 244 | Pulse | Pulse | 3.404 | 5.861 | -1.352 | -1.923 | 0.996 | 0.000 | No Zero | 0 | -1 | 0 | 0 | 0.650 | 0.395 | 1.726 | 0.536 |
| 245 | Pulse | Pulse | -0.864 | 2.223 | -0.856 | -1.226 | 0.953 | 0.000 | No Zero | 0 | -1 | 0 | 0 | 1.077 | 1.103 | 1.927 | 0.539 |
| 246 | Pulse | Pulse | -0.466 | 1.000 | -0.448 | -0.448 | 1.000 | -0.300 | -0.592 | 0 | -1 | 0 | 0 | 0.531 | 0.620 | 1.115 | 0.756 |
| 247 | Pulse | Pulse | -0.468 | 3.054 | -0.696 | -0.696 | 1.000 | -0.151 | -2.181 | 0 | -1 | 0 | 0 | 0.492 | 1.352 | 0.523 | 1.923 |

| | | | | | | | | | | | | | | | | | |
|---|---|---|---|---|---|---|---|---|---|---|---|---|---|---|---|---|---|
| 248 | Does not pulse | Pulse | 1.861 | 2.773 | -1.251 | -3.333 | 0.946 | -1.932 | -1.438 | 0 | -1 | 0 | 0 | 0.995 | 0.856 | 1.136 | 1.226 |
| 249 | Pulse | Pulse | -1.653 | 1.000 | -1.115 | -1.115 | 1.000 | -0.694 | -1.684 | 0 | -1 | 1 | -1 | 1.654 | 0.296 | 1.466 | 0.300 |
| 250 | Does not pulse | Pulse | -0.151 | 1.053 | -0.117 | -1.453 | 0.336 | -0.747 | -0.151 | 0 | -1 | 1 | -1 | 1.677 | 1.091 | 1.922 | 0.151 |
| 251 | Pulse | Pulse | -1.762 | 1.000 | -1.217 | -1.217 | 1.000 | -0.776 | -1.764 | 0 | -1 | 1 | -1 | 1.868 | 0.719 | 0.134 | 1.932 |
| 252 | Pulse | Pulse | -0.325 | 2.391 | -1.183 | -0.72 | 0.956 | -0.185 | -3.065 | 0 | -1 | 1 | -1 | 1.299 | 0.841 | 1.193 | 0.694 |
| 253 | Pulse | Pulse | -0.112 | 3.719 | -1.625 | -1.625 | 1.000 | -1.248 | -1.511 | 0 | -1 | 1 | -1 | 0.435 | 0.076 | 0.307 | 0.747 |
| 254 | Pulse | Pulse | -3.607 | 1.000 | -1.882 | -1.882 | 1.000 | -0.971 | -3.646 | 0 | -1 | 1 | -1 | 1.754 | 0.882 | 1.276 | 0.776 |
| 255 | Pulse | Pulse | -2.763 | 1.000 | -1.68 | -1.68 | 1.000 | -0.697 | -3.928 | 0 | -1 | 1 | -1 | 1.674 | 1.533 | 0.251 | 0.185 |
| 256 | Pulse | Pulse | -2.944 | 1.000 | -1.734 | -1.734 | 1.000 | -0.001 | -3.969 | 0 | -1 | 1 | -1 | 1.321 | 0.755 | 0.216 | 1.248 |
| 257 | Pulse | Pulse | -1.448 | 1.000 | -1.133 | -1.133 | 1.000 | 0.000 | -2.933 | 0 | -1 | 1 | -1 | 1.243 | 1.823 | 1.212 | 0.971 |
| 258 | Pulse | Pulse | -3.488 | 1.000 | -1.831 | -1.831 | 1.000 | 0.000 | -3.526 | 0 | -1 | 1 | -1 | 1.153 | 1.964 | 1.037 | 0.697 |
| 259 | Pulse | Pulse | -0.231 | 1.364 | -0.272 | -0.899 | 0.746 | 0.000 | -0.232 | 0 | -1 | 1 | 0 | 1.966 | 1.984 | 1.792 | 1.483 |
| 260 | Pulse | Pulse | -0.040 | 1.032 | -0.042 | -1.193 | 0.268 | 0.001 | -0.041 | 0 | -1 | 1 | 0 | 1.329 | 1.467 | 0.872 | 0.799 |
| 261 | Pulse | Pulse | 0.063 | 1.731 | -1.115 | -0.349 | 0.865 | 0.000 | -2.632 | 0 | -1 | 1 | 0 | 0.436 | 1.763 | 1.884 | 1.898 |
| 262 | Pulse | Pulse | 1.745 | 1.000 | -1.091 | -1.091 | 1.000 | 0.000 | -1.405 | 0 | -1 | 1 | 0 | 0.213 | 0.116 | 0.327 | 1.055 |
| 263 | Pulse | Pulse | 0.375 | 1.276 | -0.072 | -1.725 | 0.649 | 0.001 | -0.070 | 0 | -1 | 1 | 0 | 0.139 | 0.020 | 0.183 | 1.215 |
| 264 | Pulse | Pulse | -0.059 | 1.085 | -1.57 | -0.101 | 0.411 | 0.000 | -3.243 | 0 | -1 | 1 | 0 | 0.112 | 1.316 | 1.152 | 0.148 |
| 265 | Pulse | Pulse | -1.483 | 1.000 | -1.34 | -1.34 | 1.000 | 0.000 | -3.740 | 0 | -1 | 1 | 0 | 0.483 | 0.702 | 0.253 | 1.479 |
| 266 | Pulse | Pulse | 1.557 | 1.000 | -0.481 | -0.481 | 1.000 | 1.885 | -1.925 | 0 | -1 | 1 | 0 | 0.891 | 0.035 | 1.363 | 1.762 |
| 267 | Pulse | Pulse | 3.888 | 4.404 | -1.194 | -0.373 | 0.989 | 0.284 | -3.134 | 0 | -1 | 1 | 0 | 0.280 | 1.622 | 0.506 | 0.049 |
| 268 | Pulse | Pulse | 10.405 | 5.245 | -0.394 | -0.394 | 1.000 | 1.282 | -1.575 | 0 | -1 | 1 | 0 | 1.061 | 1.870 | 1.539 | 0.810 |
| 269 | Pulse | Pulse | 13.363 | 11.324 | -0.063 | -0.063 | 1.000 | 0.634 | -0.256 | 0 | -1 | 1 | 1 | 1.436 | 0.963 | 0.882 | 1.885 |
| 270 | Pulse | Pulse | 13.363 | 11.324 | -0.063 | -0.063 | 1.000 | 546.105 | -0.128 | 0 | -1 | 1 | 1 | 1.158 | 1.567 | 1.430 | 0.284 |
| 271 | Pulse | Pulse | 4.206 | 1.000 | -0.318 | -0.318 | 1.000 | 1.599 | -1.271 | 0 | -1 | 1 | 1 | 1.386 | 0.787 | 0.256 | 1.282 |
| 272 | Pulse | Pulse | 9.947 | 9.065 | -1.004 | -0.623 | 0.999 | 0.384 | -3.253 | 0 | -1 | 1 | 1 | 0.995 | 0.128 | 1.047 | 0.629 |
| 273 | Pulse | Pulse | 17.775 | 12.842 | -0.065 | -0.065 | 1.000 | 1.204 | -0.256 | 0 | -1 | 1 | 1 | 1.710 | 0.018 | 0.405 | 1.761 |
| 274 | Pulse | Pulse | 6.776 | 5.094 | -0.161 | -0.161 | 1.000 | 1.513 | -0.642 | 0 | -1 | 1 | 1 | 0.436 | 0.635 | 0.688 | 1.600 |
| 275 | Pulse | Pulse | 0.197 | 1.000 | -0.429 | -0.429 | 1.000 | 0.606 | -1.717 | 0 | -1 | 1 | 1 | 1.142 | 1.626 | 0.172 | 0.384 |
| 276 | Pulse | Pulse | -1.153 | 1.332 | -2.502 | -0.884 | 0.689 | No Zero | 0.000 | 0 | -1 | 1 | 1 | 1.259 | 0.128 | 1.486 | 1.207 |
| 277 | Pulse | Pulse | -1.143 | 1.001 | -3.683 | -0.574 | 0.051 | No Zero | 0.000 | 0 | -1 | 1 | 1 | 1.597 | 0.321 | 1.476 | 1.514 |
| 278 | Pulse | Pulse | -1.238 | 1.001 | -3.123 | -0.62 | 0.038 | No Zero | 0.000 | 0 | -1 | 1 | 1 | 1.763 | 0.858 | 0.375 | 0.606 |
| 279 | Pulse | Pulse | 3.662 | 3.788 | -2.42 | -0.923 | 0.977 | No Zero | 0.000 | 0 | 0 | -1 | -1 | 0.642 | 0.884 | 0.724 | 1.251 |
| 280 | Pulse | Pulse | 0.973 | 2.711 | -0.461 | -1.198 | 0.960 | No Zero | 0.000 | 0 | 0 | -1 | -1 | 1.878 | 0.574 | 0.489 | 1.842 |
| 281 | Pulse | Pulse | -0.942 | 1.082 | -2.066 | -0.542 | 0.404 | No Zero | 0.000 | 0 | 0 | -1 | -1 | 1.852 | 0.620 | 0.153 | 1.562 |
| 282 | Pulse | Pulse | -1.139 | 1.035 | -3.118 | -0.617 | 0.269 | No Zero | 0.000 | 0 | 0 | -1 | -1 | 0.261 | 0.923 | 0.880 | 1.210 |
| 283 | Pulse | Pulse | -0.089 | 1.000 | -2.42 | -0.045 | 0.027 | No Zero | 0.000 | 0 | 0 | -1 | -1 | 0.254 | 1.198 | 0.264 | 0.231 |
| 284 | Pulse | Pulse | -0.775 | 2.330 | -3.665 | -1.83 | 0.921 | No Zero | 0.000 | 0 | 0 | -1 | -1 | 0.882 | 0.542 | 1.888 | 1.033 |
| 285 | Pulse | Pulse | -0.950 | 3.075 | -2.778 | -1.855 | 0.968 | No Zero | 0.000 | 0 | 0 | -1 | -1 | 0.891 | 0.617 | 0.939 | 1.559 |
| 286 | Pulse | Pulse | 11420.710 | 337.103 | -1.256 | -1.08 | 1.000 | No Zero | 0.000 | 0 | 0 | -1 | -1 | 0.338 | 0.045 | 1.417 | 1.210 |
| 287 | Pulse | Pulse | -0.852 | 1.008 | -1.725 | -0.432 | 0.134 | No Zero | 0.000 | 0 | 0 | -1 | -1 | 0.827 | 1.830 | 0.954 | 1.832 |
| 288 | Pulse | Pulse | 993.834 | 98.669 | -0.041 | -0.25 | 1.000 | No Zero | 0.000 | 0 | 0 | -1 | -1 | 0.994 | 1.855 | 1.407 | 1.389 |
| 289 | Pulse | Pulse | 7.281 | 7.119 | -1.228 | -0.641 | 0.998 | No Zero | 0.000 | 0 | 0 | -1 | 0 | 0.009 | 1.080 | 0.826 | 1.256 |
| 290 | Pulse | Pulse | 146.714 | 38.112 | -0.551 | -0.623 | 1.000 | No Zero | 0.000 | 0 | 0 | -1 | 0 | 1.087 | 0.432 | 1.104 | 1.725 |
| 291 | Pulse | Pulse | 1475.077 | 120.495 | -1.442 | -1.661 | 1.000 | No Zero | 0.000 | 0 | 0 | -1 | 0 | 0.010 | 0.250 | 1.550 | 0.041 |
| 292 | Pulse | Pulse | -1.509 | 1.029 | -0.769 | -1.529 | 0.264 | No Zero | 0.000 | 0 | 0 | -1 | 0 | 0.285 | 0.641 | 1.810 | 1.228 |
| 293 | Does not pulse | Does not pulse | -0.005 | 1.000 | -0.336 | -0.003 | 0.001 | No Zero | 0.007 | 0 | 0 | -1 | 0 | 0.032 | 0.623 | 0.386 | 0.551 |
| 294 | Pulse | Pulse | 7.620 | 9.217 | -1.188 | -1.031 | 1.000 | No Zero | 0.000 | 0 | 0 | -1 | 0 | 0.053 | 1.661 | 1.529 | 1.442 |
| 295 | Pulse | Pulse | 4.011 | 4.097 | -0.243 | -1.186 | 0.985 | No Zero | 0.000 | 0 | 0 | -1 | 0 | 1.645 | 1.529 | 0.241 | 0.769 |
| 296 | Does not pulse | Does not pulse | -0.128 | 1.000 | -0.911 | -0.064 | 0.000 | No Zero | 0.000 | 0 | 0 | -1 | 0 | 0.301 | 1.031 | 0.838 | 1.188 |
| 297 | Does not pulse | Does not pulse | -0.224 | 1.000 | -0.516 | -0.1118 | 0.000 | No Zero | No Zero | 0 | 0 | -1 | 0 | 0.554 | 1.186 | 1.170 | 0.243 |
| 298 | Does not pulse | Does not pulse | -0.179 | 1.000 | -0.09 | -0.49 | 0.000 | No Zero | 0.000 | 0 | 0 | -1 | 1 | 0.157 | 0.064 | 0.336 | 1.048 |
| 299 | Does not pulse | Does not pulse | -1.374 | 1.000 | -0.687 | -1.487 | 0.000 | No Zero | No Zero | 0 | 0 | -1 | 1 | 1.892 | 0.490 | 1.251 | 0.413 |

| | | | | | | | | | | | | | | | | | |
|---|---|---|---|---|---|---|---|---|---|---|---|---|---|---|---|---|---|
| 300 | Does not pulse | Does not pulse | -2.209 | 1.000 | -1.1045 | -1.216 | 0.000 | No Zero | No Zero | 0 | 0 | -1 | 1 | 0.483 | 1.487 | 0.312 | 1.646 |
| 301 | Does not pulse | Does not pulse | -0.121 | 1.000 | -1.739 | -0.06 | 0.000 | No Zero | 0.000 | 0 | 0 | -1 | 1 | 0.188 | 1.960 | 1.306 | 0.568 |
| 302 | Does not pulse | Does not pulse | -0.875 | 1.000 | -0.438 | -1.441 | 0.000 | No Zero | No Zero | 0 | 0 | -1 | 1 | 1.734 | 0.060 | 1.522 | 1.792 |
| 303 | Does not pulse | Does not pulse | -0.226 | 1.000 | -0.1139 | -1.226 | 0.000 | No Zero | No Zero | 0 | 0 | -1 | 1 | 1.238 | 1.441 | 0.928 | 1.518 |
| 304 | Does not pulse | Does not pulse | -2.148 | 1.000 | 0.132 | -0.296 | 0.000 | No Zero | -1.699 | 0 | 0 | -1 | 1 | 1.884 | 1.699 | 0.275 | 1.321 |
| 305 | Does not pulse | Does not pulse | -3.414 | 1.000 | -3.123 | -1.707 | 0.000 | No Zero | No Zero | 0 | 0 | -1 | 1 | 0.077 | 0.296 | 0.370 | 1.291 |
| 306 | Does not pulse | Does not pulse | -0.676 | 1.000 | -1.935 | -0.338 | 0.000 | No Zero | No Zero | 0 | 0 | 0 | -1 | 1.713 | 1.707 | 0.988 | 1.562 |
| 307 | Does not pulse | Does not pulse | -1.073 | 1.000 | -3.068 | -0.537 | 0.000 | No Zero | No Zero | 0 | 0 | 0 | -1 | 0.549 | 1.935 | 1.981 | 0.169 |
| 308 | Does not pulse | Does not pulse | -0.616 | 1.000 | -3.571 | -0.308 | 0.000 | No Zero | No Zero | 0 | 0 | 0 | -1 | 0.660 | 0.537 | 0.432 | 1.534 |
| 309 | Does not pulse | Does not pulse | -2.070 | 1.000 | -1.677 | -1.035 | 0.000 | No Zero | No Zero | 0 | 0 | 0 | -1 | 0.730 | 0.308 | 0.330 | 1.787 |
| 310 | Does not pulse | Does not pulse | -3.807 | 1.000 | -3.574 | -1.904 | 0.000 | No Zero | No Zero | 0 | 0 | 0 | -1 | 1.892 | 1.035 | 0.037 | 0.839 |
| 311 | Does not pulse | Does not pulse | -0.134 | 1.000 | -1.551 | -0.067 | 0.000 | No Zero | No Zero | 0 | 0 | 0 | -1 | 0.244 | 1.904 | 0.540 | 1.787 |
| 312 | Does not pulse | Does not pulse | -0.301 | 1.000 | -1.952 | -0.151 | 0.000 | No Zero | No Zero | 0 | 0 | 0 | -1 | 1.790 | 1.551 | 1.818 | 0.033 |
| 313 | Does not pulse | Does not pulse | -1.033 | 1.000 | -1.136 | -0.516 | 0.000 | No Zero | No Zero | 0 | 0 | 0 | -1 | 1.919 | 0.151 | 0.570 | 0.976 |
| 314 | Does not pulse | Does not pulse | -1.075 | 1.000 | -1.584 | -0.538 | 0.000 | No Zero | No Zero | 0 | 0 | 0 | -1 | 1.941 | 1.136 | 0.548 | 0.258 |
| 315 | Does not pulse | Does not pulse | -0.048 | 1.000 | -1.229 | -0.024 | 0.000 | No Zero | No Zero | 0 | 0 | 0 | -1 | 0.310 | 0.538 | 0.868 | 0.792 |
| 316 | Does not pulse | Does not pulse | -1.595 | 1.000 | -1.086 | -0.798 | 0.000 | No Zero | No Zero | 0 | 0 | 0 | 0 | 0.850 | 1.229 | 0.894 | 0.024 |
| 317 | Does not pulse | Does not pulse | -1.297 | 1.000 | -1.758 | -0.648 | 0.000 | No Zero | No Zero | 0 | 0 | 0 | 0 | 0.069 | 0.798 | 1.959 | 1.086 |
| 318 | Does not pulse | Does not pulse | -1.578 | 1.000 | -0.851 | -0.789 | 0.000 | No Zero | No Zero | 0 | 0 | 0 | 0 | 1.825 | 0.648 | 0.581 | 1.758 |
| 319 | Does not pulse | Does not pulse | -1.700 | 1.000 | -1.391 | -0.85 | 0.000 | No Zero | No Zero | 0 | 0 | 0 | 0 | 1.558 | 0.789 | 1.765 | 0.851 |
| 320 | Does not pulse | Does not pulse | -1.986 | 1.000 | -1.467 | -0.993 | 0.000 | No Zero | No Zero | 0 | 0 | 0 | 0 | 0.933 | 0.850 | 0.910 | 1.391 |
| 321 | Does not pulse | Does not pulse | -2.367 | 1.000 | -1.91 | -1.183 | 0.000 | No Zero | No Zero | 0 | 0 | 0 | 0 | 0.191 | 1.467 | 0.260 | 0.993 |
| 322 | Does not pulse | Does not pulse | -0.733 | 1.000 | -0.583 | -0.366 | 0.000 | No Zero | No Zero | 0 | 0 | 0 | 0 | 0.519 | 1.183 | 0.455 | 1.910 |
| 323 | Does not pulse | Does not pulse | -0.756 | 1.000 | -0.593 | -0.378 | 0.000 | No Zero | No Zero | 0 | 0 | 0 | 0 | 0.126 | 0.366 | 1.248 | 0.583 |
| 324 | Does not pulse | Does not pulse | -0.313 | 1.000 | -1.32 | -0.156 | 0.000 | No Zero | No Zero | 0 | 0 | 0 | 0 | 0.274 | 0.378 | 1.913 | 0.593 |
| 325 | Does not pulse | Does not pulse | -0.120 | 1.000 | -0.448 | -0.01 | 0.000 | No Zero | No Zero | 0 | 0 | 0 | 0 | 0.474 | 1.320 | 0.009 | 0.156 |
| 326 | Does not pulse | Does not pulse | -0.020 | 1.000 | -1.118 | 0.079 | 0.000 | No Zero | No Zero | 0 | 0 | 0 | 1 | 1.704 | 1.118 | 1.141 | 1.062 |
| 327 | Does not pulse | Does not pulse | -0.848 | 1.000 | -0.893 | -0.424 | 0.000 | No Zero | No Zero | 0 | 0 | 0 | 1 | 1.718 | 0.893 | 0.767 | 1.191 |
| 328 | Does not pulse | Does not pulse | -0.760 | 1.000 | -1.553 | -0.382 | 0.000 | No Zero | No Zero | 0 | 0 | 0 | 1 | 0.558 | 0.956 | 0.629 | 1.654 |
| 329 | Does not pulse | Does not pulse | -1.912 | 1.000 | -1.025 | -0.956 | 0.000 | No Zero | No Zero | 0 | 0 | 0 | 1 | 1.486 | 0.289 | 0.137 | 1.064 |
| 330 | Does not pulse | Does not pulse | -0.577 | 1.000 | -0.928 | -0.289 | 0.000 | No Zero | No Zero | 0 | 0 | 0 | 1 | 0.374 | 1.450 | 1.767 | 1.596 |
| 331 | Does not pulse | Does not pulse | -0.670 | 1.000 | -1.671 | -0.334 | 0.000 | No Zero | No Zero | 0 | 0 | 1 | -1 | 1.686 | 1.076 | 0.419 | 1.061 |
| 332 | Does not pulse | Pulse | -2.024 | 1.102 | -2.122 | -1.076 | 0.454 | No Zero | -2.152 | 0 | 0 | 1 | -1 | 1.687 | 0.431 | 1.433 | 1.725 |
| 333 | Does not pulse | Pulse | -0.759 | 1.032 | -3.451 | -0.431 | 0.254 | No Zero | -0.861 | 0 | 0 | 1 | -1 | 0.943 | 0.921 | 1.885 | 1.257 |
| 334 | Does not pulse | Pulse | -1.232 | 1.334 | -2.513 | -0.921 | 0.691 | No Zero | -1.842 | 0 | 0 | 1 | -1 | 1.613 | 0.803 | 0.643 | 0.758 |
| 335 | Does not pulse | Pulse | -1.452 | 1.166 | -1.515 | -0.803 | 0.569 | No Zero | -1.606 | 0 | 0 | 1 | -1 | 1.438 | 0.386 | 0.980 | 0.242 |
| 336 | Does not pulse | Pulse | -0.599 | 1.499 | -0.483 | -0.386 | 0.933 | No Zero | -0.772 | 0 | 0 | 1 | -1 | 0.280 | 1.894 | 1.262 | 0.877 |
| 337 | Does not pulse | Pulse | -0.908 | 4.678 | -1.755 | -1.894 | 0.999 | No Zero | -3.789 | 0 | 0 | 1 | -1 | 1.416 | 1.059 | 1.305 | 1.556 |
| 338 | Does not pulse | Pulse | -1.777 | 1.151 | -3.111 | -1.059 | 0.515 | No Zero | -2.119 | 0 | 0 | 1 | -1 | 1.236 | 1.004 | 0.971 | 0.220 |
| 339 | Does not pulse | Pulse | -0.744 | 1.176 | -0.441 | -1.004 | 0.595 | No Zero | -2.008 | 0 | 0 | 1 | -1 | 1.833 | 0.865 | 0.854 | 0.059 |
| 340 | Does not pulse | Pulse | -0.219 | 1.016 | -0.117 | -0.865 | 0.201 | No Zero | -1.731 | 0 | 0 | 1 | -1 | 1.021 | 1.927 | 0.551 | 1.487 |
| 341 | Does not pulse | Pulse | -3.276 | 1.449 | -2.973 | -1.927 | 0.765 | No Zero | -3.855 | 0 | 0 | 1 | 0 | 0.234 | 1.539 | 1.531 | 1.082 |
| 342 | Does not pulse | Pulse | -1.022 | 2.427 | -1.082 | -1.539 | 0.958 | No Zero | -3.077 | 0 | 0 | 1 | 0 | 0.339 | 1.860 | 0.416 | 0.040 |
| 343 | Does not pulse | Pulse | -0.032 | 1.023 | -0.04 | -1.86 | 0.223 | No Zero | -3.720 | 0 | 0 | 1 | 0 | 1.203 | 1.215 | 0.938 | 1.193 |
| 344 | Does not pulse | Pulse | -1.469 | 3.113 | -1.193 | -1.215 | 1.000 | No Zero | -2.429 | 0 | 0 | 1 | 0 | 1.447 | 0.816 | 1.195 | 0.851 |
| 345 | Does not pulse | Pulse | -0.472 | 3.428 | -0.851 | -0.816 | 1.000 | No Zero | -1.632 | 0 | 0 | 1 | 0 | 0.244 | 0.700 | 1.093 | 0.254 |
| 346 | Does not pulse | Pulse | 0.227 | 1.987 | -0.254 | -0.7 | 0.926 | No Zero | -1.400 | 0 | 0 | 1 | 0 | 0.163 | 0.579 | 1.354 | 0.914 |
| 347 | Does not pulse | Pulse | -0.098 | 2.538 | -0.914 | -0.579 | 0.971 | No Zero | -1.158 | 0 | 0 | 1 | 0 | 0.998 | 0.117 | 0.147 | 0.676 |
| 348 | Does not pulse | Pulse | -0.215 | 1.025 | -0.676 | -0.117 | 0.255 | No Zero | -0.234 | 0 | 0 | 1 | 0 | 0.672 | 1.970 | 1.503 | 1.293 |
| 349 | Does not pulse | Pulse | -1.614 | 1.995 | -1.293 | -1.97 | 0.912 | No Zero | -3.939 | 0 | 0 | 1 | 0 | 1.766 | 1.024 | 0.752 | 1.768 |
| 350 | Does not pulse | Pulse | -1.733 | 1.322 | -1.768 | -1.024 | 0.711 | No Zero | -2.048 | 0 | 0 | 1 | 0 | 0.492 | 0.328 | 1.317 | 0.511 |
| 351 | Does not pulse | Pulse | 0.491 | 2.975 | -0.511 | -0.328 | 0.990 | No Zero | -0.656 | 0 | 0 | 1 | 1 | 1.194 | 1.087 | 0.260 | 1.104 |

| | | | | | | | | | | | | | | | | | |
|---|---|---|---|---|---|---|---|---|---|---|---|---|---|---|---|---|---|
| 352 | Does not pulse | Does not pulse | -1.639 | 1.000 | -0.819 | -1.087 | 0.000 | No Zero | No Zero | 0 | 1 | -1 | -1 | 0.080 | 1.932 | 1.776 | 1.278 |
| 353 | Does not pulse | Does not pulse | -1.170 | 1.000 | -0.589 | -0.933 | 0.000 | No Zero | -1.866 | 0 | 1 | -1 | -1 | 0.022 | 1.955 | 0.771 | 0.799 |
| 354 | Does not pulse | Does not pulse | -0.880 | 1.000 | -0.441 | -1.412 | 0.000 | No Zero | No Zero | 0 | 1 | -1 | -1 | 1.021 | 1.103 | 1.918 | 1.711 |
| 355 | Pulse | Pulse | 26.413 | 8.535 | -2.244 | -2.244 | 1.000 | -3.832 | 0.000 | 0 | 1 | -1 | -1 | 0.953 | 1.756 | 0.780 | 0.098 |
| 356 | Pulse | Pulse | 67.766 | 23.687 | -1.777 | -1.777 | 1.000 | -2.398 | 0.000 | 0 | 1 | -1 | -1 | 0.615 | 0.640 | 0.923 | 0.976 |
| 357 | Pulse | Pulse | -2.063 | 1.000 | -2.263 | -2.263 | 1.000 | -5.133 | 0.000 | 0 | 1 | -1 | -1 | 1.413 | 0.735 | 1.883 | 0.536 |
| 358 | Pulse | Pulse | -0.213 | 1.272 | -1.636 | -0.317 | 0.652 | -0.295 | 0.001 | 0 | 1 | -1 | -1 | 1.491 | 1.818 | 1.169 | 1.813 |
| 359 | Pulse | Pulse | -1.220 | 1.000 | -1.297 | -1.297 | 1.000 | -2.929 | 0.001 | 0 | 1 | -1 | -1 | 0.113 | 1.113 | 0.006 | 0.306 |
| 360 | Pulse | Pulse | -0.623 | 1.000 | -0.904 | -0.904 | 1.000 | -1.609 | 0.000 | 0 | 1 | -1 | -1 | 0.815 | 0.467 | 1.071 | 0.623 |
| 361 | Pulse | Pulse | -3.498 | 1.000 | -2.722 | -2.722 | 1.000 | -5.441 | -0.001 | 0 | 1 | -1 | -1 | 1.417 | 1.174 | 0.478 | 0.128 |
| 362 | Pulse | Pulse | 1.212 | 1.596 | -0.863 | -0.863 | 1.000 | -0.919 | 0.000 | 0 | 1 | -1 | 0 | 0.007 | 0.378 | 0.982 | 1.233 |
| 363 | Pulse | Pulse | -0.810 | 1.001 | -0.857 | -0.857 | 1.000 | -1.871 | 0.000 | 0 | 1 | -1 | 0 | 0.246 | 0.266 | 0.628 | 0.176 |
| 364 | Pulse | Pulse | 0.170 | 2.345 | -0.96 | -0.47 | 0.952 | -0.384 | 0.000 | 0 | 1 | -1 | 0 | 0.818 | 0.565 | 1.261 | 0.440 |
| 365 | Pulse | Pulse | 67.581 | 25.779 | -0.806 | -0.806 | 1.000 | -2.466 | 0.000 | 0 | 1 | -1 | 0 | 1.309 | 0.387 | 0.189 | 1.837 |
| 366 | Pulse | Pulse | -0.336 | 1.001 | -0.221 | -0.221 | 1.000 | -0.351 | 0.000 | 0 | 1 | -1 | 0 | 1.116 | 0.835 | 0.221 | 1.105 |
| 367 | Pulse | Pulse | -0.475 | 1.001 | -0.502 | -0.502 | 1.000 | -0.879 | 0.000 | 0 | 1 | -1 | 0 | 0.223 | 0.472 | 0.277 | 0.656 |
| 368 | Pulse | Pulse | -0.584 | 1.000 | -1.112 | -1.112 | 1.000 | -3.674 | 0.000 | 0 | 1 | -1 | 0 | 0.693 | 1.858 | 1.777 | 1.580 |
| 369 | Pulse | Pulse | -1.545 | 1.000 | -0.97 | -0.97 | 1.000 | -2.212 | 0.000 | 0 | 1 | -1 | 0 | 0.149 | 0.840 | 0.793 | 0.826 |
| 370 | Pulse | Pulse | 0.056 | 1.000 | -0.564 | -0.564 | 1.000 | -1.313 | 0.000 | 0 | 1 | -1 | 0 | 1.948 | 0.476 | 0.217 | 1.600 |
| 371 | Pulse | Pulse | 0.119 | 1.001 | -1.719 | -1.719 | 1.000 | -3.161 | 0.000 | 0 | 1 | -1 | 0 | 0.090 | 1.920 | 1.603 | 1.921 |
| 372 | Pulse | Pulse | 2.841 | 1.000 | -0.833 | -0.833 | 1.000 | -1.652 | 0.000 | 0 | 1 | -1 | 1 | 1.531 | 1.216 | 1.978 | 1.125 |
| 373 | Pulse | Pulse | -0.155 | 1.000 | -1.038 | -1.038 | 1.000 | -3.200 | 0.000 | 0 | 1 | -1 | 1 | 0.992 | 0.506 | 0.392 | 0.985 |
| 374 | Pulse | Pulse | 37.186 | 6.539 | -1.921 | -1.921 | 1.000 | -3.841 | 0.000 | 0 | 1 | -1 | 1 | 1.422 | 1.975 | 0.669 | 0.440 |
| 375 | Pulse | Pulse | 0.158 | 1.000 | -0.608 | -0.608 | 1.000 | -1.125 | 0.000 | 0 | 1 | -1 | 1 | 0.691 | 0.183 | 1.263 | 0.756 |
| 376 | Pulse | Pulse | 0.198 | 1.000 | -0.253 | -0.253 | 1.000 | -0.985 | 0.000 | 0 | 1 | -1 | 1 | 1.775 | 0.853 | 1.782 | 0.448 |
| 377 | Pulse | Pulse | 0.160 | 2.491 | -1.312 | -0.663 | 0.953 | -0.440 | 0.001 | 0 | 1 | -1 | 1 | 1.594 | 1.717 | 0.854 | 1.178 |
| 378 | Pulse | Pulse | 0.340 | 1.000 | -0.092 | -0.092 | 1.000 | -0.756 | 0.000 | 0 | 1 | -1 | 1 | 0.183 | 0.501 | 1.188 | 1.041 |
| 379 | Pulse | Pulse | 0.924 | 1.000 | -0.427 | -0.427 | 1.000 | -0.448 | 0.000 | 0 | 1 | -1 | 1 | 1.828 | 1.327 | 0.999 | 1.270 |
| 380 | Pulse | Pulse | 0.031 | 1.000 | -0.858 | -0.858 | 1.000 | -1.178 | 0.001 | 0 | 1 | -1 | 1 | 0.173 | 0.082 | 1.503 | 0.648 |
| 381 | Pulse | Pulse | 2.207 | 1.000 | -0.251 | -0.251 | 1.000 | -1.041 | 0.000 | 0 | 1 | -1 | 1 | 0.133 | 1.847 | 0.109 | 0.136 |
| 382 | Pulse | Pulse | 0.281 | 1.000 | -0.663 | -0.663 | 1.000 | -1.270 | 0.000 | 0 | 1 | 0 | -1 | 1.147 | 0.878 | 0.055 | 0.099 |
| 383 | Pulse | Pulse | 0.058 | 1.000 | -0.043 | -0.043 | 1.000 | -0.648 | -0.003 | 0 | 1 | 0 | -1 | 0.477 | 0.255 | 1.261 | 0.953 |
| 384 | Pulse | Pulse | 0.700 | 1.551 | -1.699 | -0.148 | 0.793 | -0.136 | 0.000 | 0 | 1 | 0 | -1 | 0.220 | 0.871 | 1.804 | 1.132 |
| 385 | Does not pulse | Pulse | 0.256 | 1.689 | -0.878 | -0.199 | 0.860 | -0.298 | No Zero | 0 | 1 | 0 | -1 | 1.461 | 1.962 | 1.176 | 1.006 |
| 386 | Does not pulse | Pulse | -0.442 | 1.036 | -0.255 | -1.906 | 0.278 | -2.859 | No Zero | 0 | 1 | 0 | -1 | 1.063 | 1.213 | 1.529 | 1.201 |
| 387 | Does not pulse | Pulse | -1.724 | 1.011 | -0.871 | -2.264 | 0.156 | -3.395 | No Zero | 0 | 1 | 0 | -1 | 1.445 | 0.870 | 1.293 | 0.353 |
| 388 | Does not pulse | Pulse | -2.512 | 3.707 | -1.962 | -2.013 | 0.999 | -3.019 | No Zero | 0 | 1 | 0 | -1 | 1.753 | 0.503 | 0.713 | 0.607 |
| 389 | Does not pulse | Pulse | -2.019 | 1.286 | -1.213 | -2.403 | 0.666 | -3.604 | No Zero | 0 | 1 | 0 | -1 | 1.936 | 0.385 | 0.196 | 1.388 |
| 390 | Does not pulse | Pulse | -0.123 | 3.208 | -0.87 | -0.707 | 0.994 | -1.060 | No Zero | 0 | 1 | 0 | -1 | 0.192 | 0.399 | 1.214 | 1.419 |
| 391 | Does not pulse | Pulse | 0.174 | 2.152 | -0.503 | -1.214 | 0.927 | -1.821 | No Zero | 0 | 1 | 0 | -1 | 1.781 | 1.205 | 1.725 | 1.352 |
| 392 | Does not pulse | Pulse | -0.084 | 1.262 | -0.385 | -2.775 | 0.629 | -4.162 | No Zero | 0 | 1 | 0 | 0 | 1.570 | 1.073 | 0.009 | 0.397 |
| 393 | Does not pulse | Pulse | -0.790 | 1.003 | -0.399 | -2.838 | 0.078 | -4.257 | No Zero | 0 | 1 | 0 | 0 | 0.877 | 1.117 | 0.770 | 1.294 |
| 394 | Does not pulse | Pulse | -1.582 | 1.475 | -1.205 | -2.704 | 0.765 | -4.056 | No Zero | 0 | 1 | 0 | 0 | 1.171 | 1.533 | 0.349 | 1.006 |
| 395 | Does not pulse | Pulse | 0.239 | 2.053 | -1.073 | -0.397 | 0.918 | -0.794 | No Zero | 0 | 1 | 0 | 0 | 0.765 | 1.954 | 1.872 | 1.785 |
| 396 | Does not pulse | Pulse | -1.515 | 2.391 | -1.117 | -1.294 | 0.980 | -2.587 | No Zero | 0 | 1 | 0 | 0 | 0.887 | 1.503 | 1.819 | 0.747 |
| 397 | Does not pulse | Pulse | -1.255 | 1.925 | -1.533 | -1.006 | 0.912 | -2.012 | No Zero | 0 | 1 | 0 | 0 | 0.233 | 1.050 | 0.682 | 1.699 |
| 398 | Does not pulse | Pulse | -2.956 | 2.246 | -1.954 | -1.785 | 0.976 | -3.571 | No Zero | 0 | 1 | 0 | 0 | 0.372 | 0.417 | 1.061 | 0.169 |
| 399 | Does not pulse | Pulse | -1.084 | 1.410 | -1.503 | -0.747 | 0.761 | -1.493 | No Zero | 0 | 1 | 0 | 0 | 0.482 | 1.269 | 0.222 | 1.215 |
| 400 | Does not pulse | Pulse | -2.060 | 1.047 | -1.05 | -1.699 | 0.338 | -3.397 | No Zero | 0 | 1 | 0 | 0 | 1.780 | 0.981 | 0.627 | 1.524 |
| 401 | Does not pulse | Pulse | -0.138 | 1.407 | -0.417 | -0.169 | 0.831 | -0.337 | No Zero | 0 | 1 | 0 | 0 | 1.909 | 1.292 | 0.971 | 0.876 |
| 402 | Does not pulse | Pulse | -1.999 | 2.161 | -1.269 | -1.215 | 0.994 | -2.429 | No Zero | 0 | 1 | 1 | -1 | 1.368 | 1.094 | 1.972 | 0.425 |
| 403 | Does not pulse | Pulse | -0.645 | 2.479 | -0.981 | -1.524 | 0.956 | -3.049 | No Zero | 0 | 1 | 1 | -1 | 1.838 | 1.330 | 1.487 | 0.757 |

| | | | | | | | | | | | | | | | | | |
|---|---|---|---|---|---|---|---|---|---|---|---|---|---|---|---|---|---|
| 404 | Does not pulse | Pulse | -0.214 | 2.908 | -1.292 | -0.876 | 0.977 | -1.753 | No Zero | 0 | 1 | 1 | -1 | 0.950 | 0.213 | 1.768 | 0.890 |
| 405 | Does not pulse | Pulse | -0.220 | 1.211 | -1.665 | -0.28 | 0.595 | -1.277 | -2.187 | 0 | 1 | 1 | -1 | 1.336 | 1.456 | 0.571 | 1.187 |
| 406 | Does not pulse | Pulse | -0.452 | 1.169 | -0.415 | -2.43 | 0.539 | -2.272 | -2.660 | 0 | 1 | 1 | -1 | 0.741 | 1.591 | 0.147 | 1.985 |
| 407 | Does not pulse | Pulse | -0.049 | 1.075 | -0.1 | -1.893 | 0.386 | -2.671 | -0.425 | 0 | 1 | 1 | -1 | 1.395 | 1.770 | 0.931 | 0.743 |
| 408 | Does not pulse | Pulse | -1.045 | 1.000 | -0.523 | -3.309 | 0.015 | -3.562 | -2.913 | 0 | 1 | 1 | -1 | 1.360 | 1.310 | 0.824 | 0.953 |
| 409 | Does not pulse | Pulse | -0.021 | 1.280 | -0.642 | -4.921 | 0.636 | -5.958 | -3.182 | 0 | 1 | 1 | -1 | 0.777 | 0.904 | 0.054 | 0.851 |
| 410 | Does not pulse | Pulse | -0.901 | 1.017 | -2.784 | -0.473 | 0.192 | -2.230 | -3.539 | 1 | -1 | 0 | -1 | 0.352 | 0.561 | 1.755 | 1.748 |
| 411 | Does not pulse | Pulse | 0.005 | 1.010 | -2.004 | 0 | 0.028 | -0.018 | -3.998 | 1 | -1 | 0 | -1 | 0.979 | 1.213 | 1.435 | 0.280 |
| 412 | Does not pulse | Pulse | -0.861 | 1.017 | -0.451 | -2.764 | 0.188 | -2.858 | -2.620 | 1 | -1 | 0 | -1 | 1.166 | 0.390 | 0.127 | 0.128 |
| 413 | Does not pulse | Pulse | -0.667 | 1.006 | -0.339 | -2.266 | 0.110 | -2.552 | -1.808 | 1 | -1 | 0 | -1 | 1.168 | 0.625 | 1.344 | 0.794 |
| 414 | does not pulse | Does not pulse | -0.420 | 1.000 | -0.135 | -1.697 | 0.000 | -0.848 | No Zero | 1 | -1 | 0 | -1 | 0.439 | 0.482 | 0.773 | 0.067 |
| 415 | Does not pulse | Does not pulse | -0.420 | 1.000 | -0.21 | -3.496 | 0.000 | -1.748 | No Zero | 1 | -1 | 0 | -1 | 0.693 | 1.104 | 1.117 | 0.134 |
| 416 | Does not pulse | Does not pulse | -1.120 | 1.000 | -0.78 | -0.56 | 0.000 | -0.280 | No Zero | 1 | -1 | 0 | 0 | 0.380 | 1.923 | 1.070 | 1.829 |
| 417 | Does not pulse | Does not pulse | -1.920 | 1.000 | -1.051 | -0.96 | 0.000 | No Zero | No Zero | 1 | -1 | 0 | 0 | 0.393 | 1.055 | 0.295 | 0.146 |
| 418 | Does not pulse | Does not pulse | -1.280 | 1.000 | -1.1542 | -0.64 | 0.000 | No Zero | No Zero | 1 | -1 | 0 | 0 | 1.110 | 1.963 | 0.326 | 0.313 |
| 419 | Does not pulse | Does not pulse | -0.268 | 1.000 | -0.352 | -0.134 | 0.000 | -0.067 | No Zero | 1 | -1 | 0 | 0 | 1.020 | 1.210 | 1.766 | 0.244 |
| 420 | Does not pulse | Does not pulse | -0.535 | 1.000 | -0.864 | -0.267 | 0.000 | -0.134 | No Zero | 1 | -1 | 0 | 0 | 0.370 | 1.537 | 1.795 | 1.037 |
| 421 | Does not pulse | Does not pulse | -2.547 | 1.000 | -1.274 | -1.829 | 0.000 | No Zero | No Zero | 1 | -1 | 0 | 0 | 1.689 | 0.458 | 0.857 | 0.737 |
| 422 | Does not pulse | Does not pulse | -0.293 | 1.000 | -0.861 | -0.146 | 0.000 | 0.000 | No Zero | 1 | -1 | 0 | 0 | 1.392 | 1.889 | 0.436 | 1.506 |
| 423 | Does not pulse | Does not pulse | -0.626 | 1.000 | -0.896 | -0.313 | 0.000 | 0.000 | No Zero | 1 | -1 | 0 | 1 | 1.754 | 0.323 | 0.707 | 0.116 |
| 424 | Does not pulse | Does not pulse | -0.488 | 1.000 | -1.069 | -0.244 | 0.000 | 0.000 | No Zero | 1 | -1 | 1 | -1 | 0.888 | 0.882 | 0.653 | 1.829 |
| 425 | Does not pulse | Does not pulse | -2.073 | 1.000 | -1.324 | -1.037 | 0.000 | 0.000 | No Zero | 1 | -1 | 1 | -1 | 0.989 | 1.420 | 1.329 | 1.664 |
| 426 | Does not pulse | Does not pulse | -1.400 | 1.000 | -1.98 | -0.74 | 0.000 | No Zero | No Zero | 1 | -1 | 1 | -1 | 0.516 | 1.538 | 0.821 | 0.111 |
| 427 | Does not pulse | Does not pulse | -2.560 | 1.000 | -1.55 | -1.28 | 0.000 | No Zero | No Zero | 1 | -1 | 1 | -1 | 1.741 | 1.945 | 0.234 | 1.017 |
| 428 | Does not pulse | Pulse | 0.436 | 1.507 | -0.513 | -3.145 | 0.766 | -1.829 | -0.882 | 1 | -1 | 1 | -1 | 1.511 | 0.220 | 0.068 | 0.882 |
| 429 | Does not pulse | Pulse | 0.067 | 2.323 | -1.028 | -2.3 | 0.927 | -1.664 | -1.420 | 1 | -1 | 1 | -1 | 0.260 | 1.943 | 1.880 | 1.866 |
| 430 | Pulse | Pulse | 2.166 | 2.998 | -0.111 | -0.111 | 1.000 | -0.111 | -1.538 | 1 | -1 | 1 | -1 | 1.968 | 1.386 | 1.405 | 0.743 |
| 431 | Pulse | Pulse | 5.552 | 8.387 | -1.017 | -1.017 | 1.000 | -1.017 | -1.945 | 1 | -1 | 1 | -1 | 0.128 | 0.887 | 1.086 | 1.080 |
| 432 | Does not pulse | Pulse | 17.991 | 1.001 | -0.118 | -1.647 | 0.997 | -0.882 | -0.220 | 1 | -1 | 1 | -1 | 1.573 | 1.203 | 1.894 | 1.262 |
| 433 | Does not pulse | Pulse | 10.583 | 11.392 | -1.866 | -1.866 | 1.000 | -1.866 | -1.943 | 1 | -1 | 1 | -1 | 1.758 | 0.245 | 1.627 | 1.955 |
| 434 | Pulse | Pulse | 0.002 | 1.000 | -0.742 | -0.742 | 1.000 | -0.743 | -1.386 | 1 | -1 | 1 | 0 | 0.462 | 1.825 | 1.353 | 1.450 |
| 435 | Does not pulse | Pulse | 5.534 | 5.371 | -0.623 | -1.537 | 0.993 | -1.080 | -0.887 | 1 | -1 | 1 | 0 | 1.372 | 1.593 | 1.059 | 1.509 |
| 436 | Does not pulse | Pulse | 0.032 | 3.095 | -0.988 | -1.537 | 0.977 | -1.262 | -1.203 | 1 | -1 | 1 | 0 | 1.007 | 1.814 | 0.247 | 1.704 |
| 437 | does not pulse | Pulse | 0.431 | 1.177 | -0.127 | -3.784 | 0.539 | -1.955 | -0.245 | 1 | -1 | 1 | 0 | 0.350 | 1.528 | 0.919 | 1.212 |
| 438 | Pulse | Pulse | 0.120 | 1.000 | -0.725 | -0.725 | 1.000 | -0.001 | -1.825 | 1 | -1 | 1 | 0 | 0.728 | 0.804 | 1.460 | 1.910 |
| 439 | Pulse | Pulse | 0.430 | 1.000 | -0.754 | -0.754 | 1.000 | 0.002 | -1.593 | 1 | -1 | 1 | 0 | 1.758 | 1.219 | 1.936 | 1.268 |
| 440 | Pulse | Pulse | 10.673 | 1.000 | -0.852 | -0.852 | 1.000 | 0.000 | -1.814 | 1 | -1 | 1 | 0 | 1.555 | 1.797 | 0.453 | 0.203 |
| 441 | Pulse | Pulse | 0.423 | 1.000 | -0.606 | -0.606 | 1.000 | 0.000 | -1.528 | 1 | -1 | 1 | 0 | 1.657 | 0.849 | 1.454 | 1.873 |
| 442 | Pulse | Pulse | 0.043 | 1.000 | -0.955 | -0.955 | 1.000 | 0.000 | -0.804 | 1 | -1 | 1 | 0 | 0.593 | 0.624 | 1.099 | 1.105 |
| 443 | Pulse | Pulse | 0.435 | 1.000 | -0.634 | -0.634 | 1.000 | 0.000 | -1.219 | 1 | -1 | 1 | 0 | 1.281 | 1.193 | 0.322 | 0.836 |
| 444 | Pulse | Pulse | 0.204 | 1.000 | -0.101 | -0.101 | 1.000 | 0.000 | -1.797 | 1 | -1 | 1 | 1 | 0.738 | 0.161 | 0.473 | 1.989 |
| 445 | Pulse | Pulse | 0.035 | 1.000 | -0.937 | -0.937 | 1.000 | 0.000 | -0.849 | 1 | -1 | 1 | 1 | 1.819 | 1.582 | 0.270 | 1.101 |
| 446 | Pulse | Pulse | 0.096 | 1.000 | -0.553 | -0.553 | 1.000 | 0.000 | -0.624 | 1 | -1 | 1 | 1 | 0.108 | 1.353 | 1.645 | 1.823 |
| 447 | Pulse | Pulse | 2.059 | 1.000 | -0.418 | -0.418 | 1.000 | 0.000 | -1.193 | 1 | -1 | 1 | 1 | 0.294 | 0.610 | 1.560 | 0.974 |
| 448 | does not pulse | Pulse | 878.291 | 88.070 | -0.16 | -1.344 | 1.000 | -0.700 | -0.161 | 1 | -1 | 1 | 1 | 1.098 | 1.756 | 1.977 | 0.038 |
| 449 | Pulse | Pulse | 1.856 | 4.034 | -0.2 | -0.2 | 1.000 | -0.608 | -1.582 | 1 | -1 | 1 | 1 | 0.703 | 1.069 | 1.496 | 1.940 |
| 450 | Pulse | Pulse | -0.045 | 4.160 | -0.865 | -0.865 | 1.000 | 0.849 | -1.353 | 1 | -1 | 1 | 1 | 1.390 | 0.547 | 1.902 | 1.815 |
| 451 | Pulse | Pulse | 1.091 | 1.000 | -0.023 | -0.023 | 1.000 | 0.050 | -0.610 | 1 | -1 | 1 | 1 | 0.915 | 1.466 | 1.116 | 1.988 |
| 452 | Pulse | Pulse | -0.042 | 1.000 | -0.596 | -0.596 | 1.000 | 0.000 | 0.000 | 1 | -1 | 1 | 1 | 0.779 | 1.763 | 1.787 | 0.772 |
| 453 | Pulse | Pulse | -0.042 | 1.000 | -0.596 | -0.596 | 1.000 | -0.041 | -1.466 | 1 | -1 | 1 | 1 | 1.455 | 1.825 | 1.808 | 0.163 |
| 454 | Pulse | Pulse | -0.031 | 1.021 | -0.72 | -0.72 | 1.000 | -0.444 | -1.763 | 1 | 0 | -1 | 0 | 0.513 | 0.108 | 1.313 | 0.555 |
| 455 | Pulse | Pulse | 4.751 | 3.840 | -1.361 | -0.101 | 0.979 | 0.023 | -1.825 | 1 | 0 | -1 | 0 | 1.418 | 0.261 | 1.048 | 0.092 |

| | | | | | | | | | | | | | | | | | |
|---|---|---|---|---|---|---|---|---|---|---|---|---|---|---|---|---|---|
| 456 | Does not pulse | Does not pulse | -2.663 | 1.000 | -3.246 | -1.331 | 0.000 | No Zero | No Zero | 1 | 0 | -1 | 0 | 1.610 | 0.356 | 0.483 | 1.189 |
| 457 | Does not pulse | Does not pulse | -1.530 | 1.000 | -0.787 | -0.765 | 0.000 | No Zero | No Zero | 1 | 0 | 0 | -1 | 0.439 | 1.770 | 0.098 | 1.624 |
| 458 | Does not pulse | Does not pulse | -1.530 | 1.000 | -2.455 | 1.17 | 0.000 | No Zero | No Zero | 1 | 0 | 0 | -1 | 0.065 | 0.830 | 1.189 | 0.394 |
| 459 | Does not pulse | Does not pulse | -0.880 | 1.000 | -3.652 | -0.441 | 0.000 | No Zero | No Zero | 1 | 0 | 0 | -1 | 1.592 | 0.422 | 0.349 | 1.228 |
| 460 | Does not pulse | Does not pulse | -1.810 | 1.000 | -2.4425 | -0.5902 | 0.000 | No Zero | No Zero | 1 | 0 | 0 | -1 | 0.760 | 0.070 | 0.455 | 1.814 |
| 461 | Does not pulse | Does not pulse | -0.351 | 1.000 | -1.551 | -0.176 | 0.000 | No Zero | No Zero | 1 | 0 | 0 | -1 | 1.738 | 1.165 | 1.122 | 0.002 |
| 462 | Does not pulse | Does not pulse | -1.500 | 1.000 | -2.742 | -0.75 | 0.000 | No Zero | No Zero | 1 | 0 | 0 | -1 | 0.254 | 0.429 | 1.654 | 0.775 |
| 463 | Does not pulse | Does not pulse | -2.412 | 1.000 | -2.993 | -1.206 | 0.000 | No Zero | No Zero | 1 | 0 | 0 | -1 | 0.385 | 1.135 | 1.315 | 1.371 |
| 464 | Does not pulse | Does not pulse | -1.818 | 1.000 | -1.415 | -0.909 | 0.000 | No Zero | No Zero | 1 | 0 | 0 | -1 | 0.707 | 1.914 | 0.487 | 1.497 |
| 465 | Does not pulse | Does not pulse | -1.738 | 1.000 | -1.063 | -0.869 | 0.000 | No Zero | No Zero | 1 | 0 | 0 | 0 | 0.780 | 1.690 | 0.744 | 1.415 |
| 466 | Does not pulse | Does not pulse | -1.219 | 1.000 | -0.735 | -0.61 | 0.000 | No Zero | No Zero | 1 | 0 | 0 | 0 | 0.691 | 1.754 | 1.501 | 0.869 |
| 467 | Does not pulse | Does not pulse | -2.735 | 1.000 | -1.736 | -1.367 | 0.000 | No Zero | No Zero | 1 | 0 | 0 | 0 | 0.145 | 0.881 | 1.213 | 0.610 |
| 468 | Does not pulse | Does not pulse | -3.280 | 1.000 | -1.783 | -1.64 | 0.000 | No Zero | No Zero | 1 | 0 | 0 | 0 | 0.033 | 1.769 | 0.421 | 1.367 |
| 469 | Does not pulse | Does not pulse | -0.827 | 1.000 | -1.056 | -0.413 | 0.000 | No Zero | No Zero | 1 | 0 | 0 | 0 | 0.309 | 1.949 | 1.005 | 1.783 |
| 470 | Pulse | Pulse | 41.482 | 12.455 | -0.625 | -3.01 | 0.999 | -5.454 | 1.036 | 1 | 0 | 0 | 0 | 0.696 | 1.752 | 0.187 | 0.413 |
| 471 | Pulse | Pulse | 8.134 | 4.377 | -0.448 | -2.585 | 0.982 | -4.550 | 0.764 | 1 | 1 | -1 | -1 | 0.756 | 1.036 | 0.189 | 1.818 |
| 472 | Pulse | Pulse | 24.144 | 10.680 | -0.681 | -2.148 | 0.999 | -4.243 | 1.036 | 1 | 1 | -1 | -1 | 0.415 | 0.764 | 1.321 | 1.517 |
| 473 | Pulse | Pulse | 0.064 | 1.080 | -0.044 | -1.741 | 0.397 | -2.679 | 0.088 | 1 | 1 | -1 | -1 | 0.346 | 1.035 | 1.991 | 1.415 |
| 474 | Pulse | Pulse | 1.279 | 1.476 | -0.175 | -3.348 | 0.750 | -5.284 | 0.332 | 1 | 1 | -1 | -1 | 0.161 | 0.087 | 0.982 | 0.893 |
| 475 | Pulse | Pulse | 45.310 | 21.112 | -0.189 | -0.189 | 1.000 | -0.566 | 0.833 | 1 | 1 | -1 | -1 | 0.974 | 0.332 | 0.721 | 1.761 |
| 476 | Pulse | Pulse | 423.125 | 64.507 | -0.776 | -0.776 | 1.000 | -2.328 | 1.893 | 1 | 1 | -1 | -1 | 1.489 | 0.834 | 1.815 | 0.189 |
| 477 | Pulse | Pulse | 2.842 | 2.597 | -0.077 | -1.593 | 0.942 | -2.504 | 0.146 | 1 | 1 | -1 | -1 | 0.363 | 1.893 | 0.202 | 0.776 |
| 478 | Pulse | Pulse | 101.987 | 24.092 | -0.925 | -2.912 | 1.000 | -5.756 | 1.405 | 1 | 1 | -1 | -1 | 0.578 | 0.146 | 0.389 | 0.835 |
| 479 | Pulse | Pulse | 0.286 | 1.201 | -0.163 | -2.998 | 0.569 | -4.742 | 0.310 | 1 | 1 | -1 | -1 | 0.586 | 1.404 | 0.479 | 1.919 |
| 480 | Pulse | Pulse | 1.080 | 1.000 | -0.304 | -0.304 | 1.000 | -1.218 | 1.993 | 1 | 1 | -1 | -1 | 0.611 | 0.310 | 1.111 | 1.581 |
| 481 | Pulse | Pulse | 20.487 | 8.798 | -0.395 | -0.395 | 1.000 | -1.582 | 1.922 | 1 | 1 | -1 | 0 | 0.888 | 1.992 | 0.873 | 0.609 |
| 482 | Pulse | Pulse | 5.020 | 7.933 | -0.998 | -0.998 | 1.000 | -3.991 | 0.540 | 1 | 1 | -1 | 0 | 0.493 | 1.922 | 0.446 | 0.791 |
| 483 | Pulse | Pulse | 22.574 | 14.544 | -0.079 | -0.079 | 1.000 | -0.316 | 1.102 | 1 | 1 | -1 | 0 | 0.449 | 0.540 | 0.837 | 1.995 |
| 484 | Pulse | Pulse | 0.328 | 1.000 | -0.4 | -0.4 | 1.000 | -1.594 | 1.792 | 1 | 1 | -1 | 0 | 1.822 | 1.101 | 1.193 | 0.158 |
| 485 | Pulse | Pulse | 34.736 | 15.196 | -0.679 | -0.679 | 1.000 | -2.715 | 1.299 | 1 | 1 | -1 | 0 | 1.153 | 1.796 | 0.927 | 0.797 |
| 486 | Pulse | Pulse | 2.742 | 1.000 | -0.745 | -0.745 | 1.000 | -2.980 | 1.310 | 1 | 1 | -1 | 0 | 0.209 | 1.304 | 1.983 | 1.356 |
| 487 | Pulse | Pulse | 1.166 | 1.000 | -0.605 | -0.605 | 1.000 | -2.421 | 1.008 | 1 | 1 | -1 | 0 | 0.857 | 1.310 | 1.177 | 1.490 |
| 488 | Pulse | Pulse | 1.596 | 1.000 | -0.379 | -0.379 | 1.000 | -1.519 | 1.406 | 1 | 1 | -1 | 0 | 1.282 | 1.007 | 1.876 | 1.211 |
| 489 | Pulse | Pulse | 0.500 | 1.000 | -0.435 | -0.435 | 1.000 | -1.739 | 1.047 | 1 | 1 | -1 | 0 | 1.278 | 1.405 | 1.722 | 0.759 |
| 490 | Pulse | Pulse | 0.880 | 2.514 | -0.359 | -0.359 | 1.000 | -1.951 | -0.321 | 1 | 1 | -1 | 0 | 1.424 | 1.047 | 0.727 | 0.869 |
| 491 | Pulse | Pulse | 0.880 | 2.514 | -0.359 | -0.359 | 1.000 | -3.772 | -0.356 | 1 | 1 | -1 | 1 | 1.375 | 0.454 | 1.958 | 1.951 |
| 492 | Pulse | Pulse | 6.039 | 3.831 | -0.099 | -0.099 | 1.000 | -0.896 | 1.839 | 1 | 1 | -1 | 1 | 0.579 | 0.677 | 1.993 | 1.578 |
| 493 | Pulse | Pulse | 6.039 | 3.831 | -0.153 | 1.929 | 0.345 | -43.706 | 0.302 | 1 | 1 | -1 | 1 | 1.590 | 1.265 | 1.623 | 0.896 |
| 494 | Pulse | Pulse | 2.032 | 1.000 | -0.271 | -0.271 | 1.000 | -1.604 | -0.482 | 1 | 1 | -1 | 1 | 1.661 | 0.253 | 1.027 | 1.432 |
| 495 | Pulse | Pulse | -1.063 | 1.145 | -0.62 | -1.621 | 0.526 | -1.991 | -0.256 | 1 | 1 | -1 | 1 | 0.496 | 1.064 | 0.764 | 1.604 |
| 496 | Pulse | Pulse | 1.882 | 1.000 | -0.474 | -0.474 | 1.000 | -0.933 | 0.846 | 1 | 1 | -1 | 1 | 1.342 | 1.966 | 1.874 | 1.153 |
| 497 | Pulse | Pulse | 2.598 | 1.000 | -0.1931 | -0.1931 | 1.000 | -0.481 | 1.125 | 1 | 1 | -1 | 1 | 0.160 | 0.828 | 0.362 | 1.991 |
| 498 | Pulse | Pulse | -0.412 | 1.000 | -0.582 | -0.582 | 1.000 | -1.087 | -0.086 | 1 | 1 | -1 | 1 | 1.041 | 1.771 | 1.297 | 0.933 |
| 499 | Does not pulse | Does not pulse | -0.804 | 1.000 | -0.402 | -3.622 | 0.000 | No Zero | No Zero | 1 | 1 | -1 | 1 | 0.191 | 1.936 | 1.240 | 0.312 |
| 500 | Does not pulse | Does not pulse | -1.300 | 1.000 | -0.651 | -1.021 | 0.000 | -1.532 | No Zero | 1 | 1 | -1 | 1 | 0.797 | 1.765 | 1.078 | 1.087 |
| 501 | Does not pulse | Does not pulse | -1.854 | 1.000 | -0.927 | -2.36 | 0.000 | No Zero | No Zero | 1 | 1 | 0 | -1 | 0.716 | 1.612 | 1.078 | 1.180 |
| 502 | Does not pulse | Does not pulse | -1.918 | 1.000 | -0.959 | -0.3305 | 0.000 | No Zero | No Zero | 1 | 1 | 0 | -1 | 0.462 | 0.204 | 1.289 | 1.960 |
| 503 | Does not pulse | Does not pulse | -0.708 | 1.000 | -0.354 | -3.353 | 0.000 | -5.029 | No Zero | 1 | 1 | 0 | -1 | 0.203 | 0.376 | 0.019 | 1.677 |
| 504 | Does not pulse | Does not pulse | -1.260 | 1.000 | -3.759 | -0.634 | 0.000 | No Zero | No Zero | 1 | 1 | 0 | -1 | 1.088 | 1.398 | 0.158 | 1.019 |
| 505 | Does not pulse | Does not pulse | -2.340 | 1.000 | -2.68 | -1.17 | 0.000 | No Zero | No Zero | 1 | 1 | 0 | -1 | 1.214 | 0.328 | 0.798 | 1.065 |
| 506 | Does not pulse | Does not pulse | -2.660 | 1.000 | -3.79 | -1.33 | 0.000 | No Zero | No Zero | 1 | 1 | 0 | 0 | 1.750 | 1.318 | 1.575 | 0.252 |
| 507 | Does not pulse | Does not pulse | -2.538 | 1.000 | -1.618 | -1.269 | 0.000 | -2.538 | No Zero | 1 | 1 | 0 | 0 | 1.050 | 1.799 | 0.218 | 1.269 |

| | | | | | | | | | | | | | | | | | | | |
|---|---|---|---|---|---|---|---|---|---|---|---|---|---|---|---|---|---|---|---|
| 508 | Does not pulse | Does not pulse | -2.670 | 1.000 | -1.98 | -1.33 | 0.000 | No Zero | No Zero | 1 | 1 | 0 | 0 | 0.162 | 0.822 | 1.425 | 0.201 |
| 509 | Does not pulse | Does not pulse | -1.420 | 1.000 | -1.32 | -0.799 | 0.000 | No Zero | No Zero | 1 | 1 | 0 | 0 | 1.620 | 1.276 | 1.796 | 1.244 |
| | | | | | | | | | | | | | | | | | |
